# Supplementary material for: Sub-Pixel Scale Structured Illumination for Lateral Resolution Enhancement of Non-Diffraction-Limited Flow Imaging
Source: arXiv:2510.18307 ancillary file (2025-10-21)
Supplement: Supplementary file 1 [file Supplemental_Information.pdf]

# Supplemental Document for: Sub-Pixel Scale Structured Illumination for Lateral Resolution Enhancement of Non-Diffraction-Limited Flow Imaging

Hy Cao,[1,2] Abhishek Saha,[1*] Lisa V. Poulikakos[1,2 *]
[1] Department of Mechanical and Aerospace Engineering, UC San Diego, La Jolla, CA, USA
[2]Program of Materials Science and Engineering, UC San Diego, La Jolla, CA, USA

## S1 System Setup

### Setup Component Specification

The setup studied for proof of concept was produced and mounted to a Newport OTS-UT2 optical imaging table. The illumination source of the setup was a generic A4 LED drawing board from Comzler mounted to the table by 3D printed supports. The spectra of the illumination source were captured. Supplemental Figure S1 shows the spectra of the utilized illumination panel. This panel was a generic A4 drawing board illuminating broadband white light. This spectrum was captured through a Teledyne Princeton Instruments IsoPlane 160 connected to a PIXIS 400BR.
The structured light patterns generated in MATLAB were printed onto a clear PET film from UOKHO by an ink-jet Epson ET-8550 to create gratings. The Epson ET-8550 ink jet head has a1440 by 5760 dots per inch vertical by horizonal resolution. Generated photos in MATLAB were loaded into Photoshop at a resolution of 1440 dots per inch for printing. Gratings could be generated with a minimum spot pitch of 105 micron and a minimum spacing of 352 microns.

The removable holder designed for handling the grating consists of two 3D printed frames with a finger tab. These frames are connected by screws and sandwich the PET grating. Several of these were printed and made to accommodate different gratings for ease of change. The 3D printed housing that these then slide into to was designed to mount to the linear guide. The gratings are inserted from the top and its fine position adjustment can be made by positioning screws. These screws are 3 sets of 2 placed at the bottom and two sides of the housing. This housing is mounted into the linear guide and bolted down.

A FUYU FSL30 100 mm linear guide and rail are utilized for this system. It is mounted to a 3D printed base that also houses the electronics (Supplemental Figure S2). A generic LM393 photoelectric sensor from DAOKAI was mounted to the end of the linear rail and a 3D printed tab was used as a flag for the sensor. An Arduino DUO and DM320T motor controller in a 3D printed housing on the base platform. Power was supplied to each independently. The base holding all these components was then bolted to the optical table. This sub-assembly is shown in Supplemental Figure S3.

The subject platform is a separate 3D printed assembly that does not mount to other components. It consists of two 3D printed components. The main component is a complex part with multiple features. It contains a u-shape structure for mounting the glass plates as well as a rectangular well with a brim higher than that of the glass outlet. The u-shaped structure contains two channels, one on either side, in which GE household silicon sealant was applied to create a waterproof seal once the glass plates were attached. This channel is 7 mm thick with a width of 86 mm and height of 130 mm. A 6061- T6 aluminum tube with an inner diameter of 5.63 mm and length of 200 mm was attached to the 2nd 3D printed part and pushed through until it sat approximately 50 mm in front of the top of the channel. It was then sealed with silicone. A 60 ml syringe was attached to the aluminum tube using 6 mm automotive tubing and pumped using a

KDS 100 syringe pump. The second 3D printed component was needed to seal the top of the glass channel and provide a stable point for the aluminum tube to be installed. These components were also sealed with the same silicon sealant. To match the height of this component to the grating, Thorlabs half-inch optical posts were utilized. This was then mounted as close as possible to the grating to minimize the spread of light. Lastly, focus was set on the glass plate closest to the grating.

The optical train contains a Nikon 50 mm f/1.8D adapted to a Thorlabs CS165CM camera with $3.45\mu m$ by $3.45\mu m$ pixels mounted onto a Thorlabs DTS50 translation stage for fine axial translation alignment. Focus was set on the rear end of the glass channel. A LG UltraPC Laptop with an AMD Ryzen 7 5825U was utilized for computer control and image processing. The camera was controlled through ThorCam and Arduino programming was done through the Arduino IDE.

Once all components were set up, the fluid channel was filled as this affected the optical magnification. The camera was set to an 8 by 8 bin setting and alignment was run. The grating was initially set to one end of the linear stage. Vertical and horizontal alignment between the imaging sensor and grating was done, followed by rotation to ensure parallelism between the imaging plane and sensor plane. Lastly, the pixel scale was tuned utilizing the resulting Moiré effect. The grating was moved to the other end of the linear stage and alignment was adjusted to ensure system alignment through the linear range of motion. The camera was then set back to normal settings from the 8 by 8 bin to verify that the alignment technique was possible. Images were captured un-binned.

For static images, the fluid channel was kept filled to not require any adjustments between this or the flow imaging parameters. Subjects were taped to the front of the glass plate. For flow imaging, dyed water was utilized and pumped by a KDS100 syringe pump. The dye was McCormik assorted food colors in red, yellow, and blue. Green dye was created by mixing equal parts yellow and blue for the experiments. All water utilized was deionized.

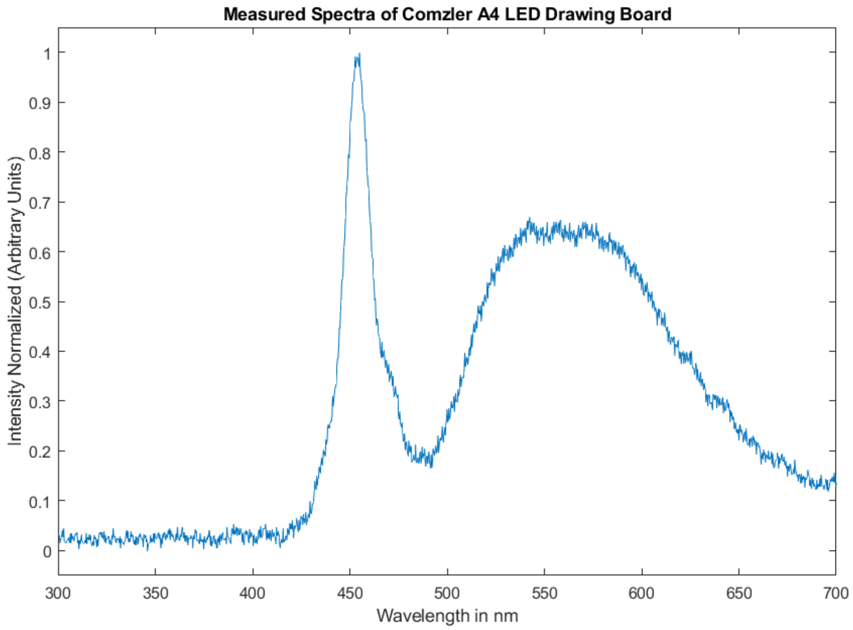


Supplemental Figure S1: Measured Spectra of Utilized Comzler A4 LED Drawing Board

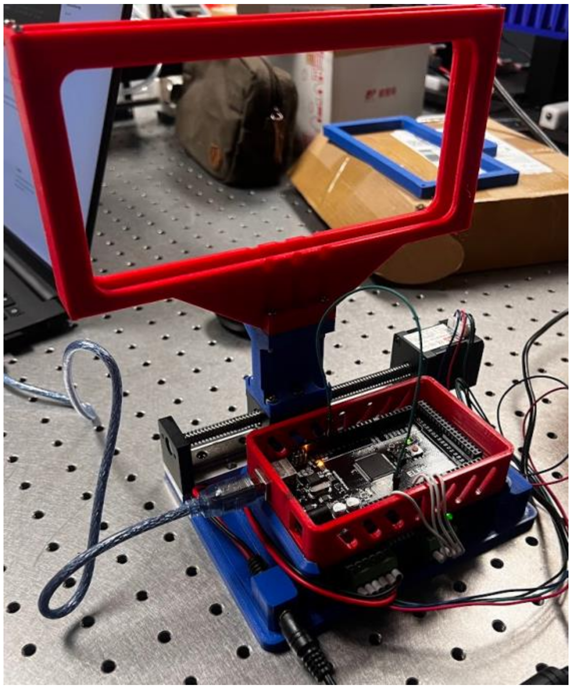

Supplemental Figure S2: Electronics and linear rail sub-assembly.

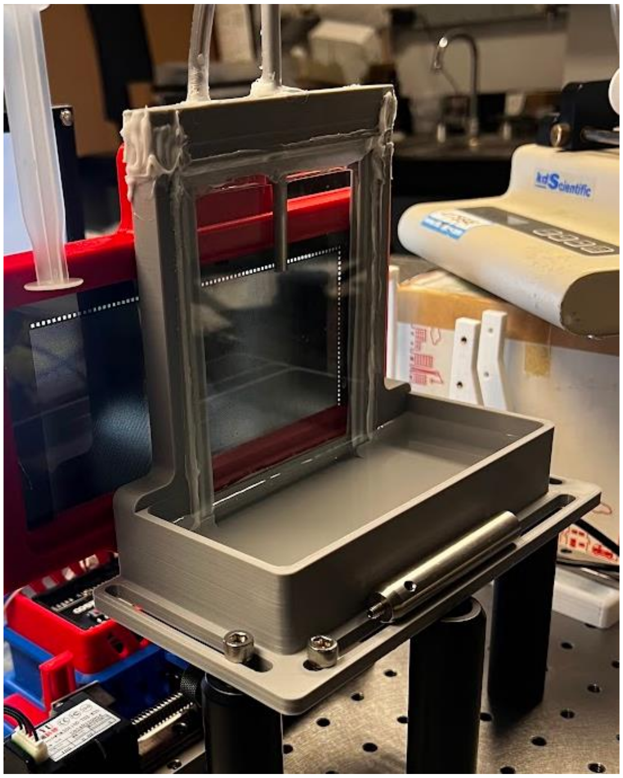


Supplemental Figure S3: Subject holder and platform for static and flow subjects.

## S 2 Flow Analysis

Supplemental Table S1 shows the parameters for additional flows captured and recombined utilizing our technique. The flows range in mass flow rate from 60 to 160 milliliters per hour. For all tests, a grating spacing of 352 microns with 105-micron holes was utilized and results in a rHR pixel scale of 176 microns. Samples for 60, 80, and 120 milliliters per hour were captured at the system running with a capture rate of 20 and 40.05 frames per second. This corresponds to a grating velocity of 3.5 and 7.06 millimeters per second, respectively. Samples for 100 and 160 milliliters per hour were captured only for a frame rate of 40.05 frames per second with a corresponding grating velocity of 7.06 millimeters per second.

All flow was generated using a 5.83 mm diameter aluminum nozzle jetting into a 7 mm width channel. With these parameters, Supplemental Table S1 contains the pixel scale, imaging frame rate, grating velocity, mass flow rate of the jet, estimated flow velocity, Reynolds number, allowable shifts per frame for the grating velocity, and estimated max shift of the flow per imaging frame for each flow tested.

As stated in the main text, captured images in camera were output as raw 16-bit color TIFF. Since green dye was used, images were debayered and the green image channels were extracted into a 16-bit monochromatic TIFF to obtain a higher signal to noise ratio. Images were then binned by a factor of 8 and separated into sets based on the grating direction changes. After reconstruction, images were scaled for contrast. The resulting pixel scale of the LR image is 352 $\mu m$ and utilizing the more conservative Nyquist–Shannon criterion results in a spatial frequency of approximately 810 $\mu m$. The resulting reconstructed HR image has four times the pixel count and a pixel scale of 176 $\mu m$ and a resulting spatial frequency of approximately 405 $\mu m$.

Supplemental Table S1 specifies the different flows captured, their varying system parameters, and estimations of the resulting flow characteristics. Figures S4 through S28 show a selection of sample images from the 7 different flow trials. Each contains the cLR and rHR image with their respective gradient images and a plot of the middle-most column of the gradient information to demonstrate the enhancement in this gradient. Each trial has 4 examples shown, the first and 401$^{st}$ image in two different sets captured consecutively with a corresponding time from initial frame in the first set. Each pair of images with the same trial and set number are cropped into the same region. This crop is done to focus on the front of the flow where the most development is occurring. Supplemental Table S2 shows specific information about the individually processed sets of data captured during each trial that was used for the following figures.

In all examples, we see a refinement in the available information of the images with a starkly more visible change in the gradients between the cLR and rHR gradient images. For every gradient line cut we see a refinement of the gradient with often sharper, taller peaks with more well-defined edges to the flow front edge. Visible in the gradients of trials 1, 2, and 4 through 7 are structures toward the center of the flow moving down and outward that are sharper and better defined after reconstruction. These all point to an increase in the available information from this technique. Specifically for flow analysis, the better refinement of the information at the edges of these flows is important as these features are the most critical in definition of the resulting flow characteristics such as boundary thickness.

Also noted is the increase in baseline noise seen in the background of every image, gradient, and in the line cuts of the gradients in the floor of the data. Perfectly horizontal or vertical

artifacts are occasionally visible as noise and likely tied to linear motion of the grating. Furthermore, when the contrast between features and background is low such as in trial 1, set 1, frame 1, noise nearly overcomes available signal, and the gradient is poorly defined.

The estimated thickness of the flow boundary at the edge of the development, as seen in the gradient images, are shown in Supplemental Table S2 under the column *Estimated Flow Thickness (mm)*. In general, we expect that as the flow speeds up, the flow developmental region at the jet tip decreases in thickness. Comparing trials 4, 5, 6, and 7 we do see a general trend of decreasing thickness going from 80 to 160 milliliters per hour flow rate. 80 ml per hour has an average thickness of 3.73 mm and 160 ml per hour has an average thickness of 3.33 mm, showing the expected trend. When we analyze trials 1, 2 and 3, it does not conform to expected results and trends in the opposite direction with much greater variability in between the four estimated samples within each trial. This may be due to poor flow conditions as seen in both trials 2 and 3, where trial 2 has poor contrast leading to inaccuracies in measurement and trial 3 contains disruptions in the flow. A smaller pixel scale may also contribute to increased accuracy of the flow thickness measurement but was limited in this setup due to the grating sizes.

Supplemental Table S1: Flow trial initial parameters and estimated flow characteristic values.

| Flow Trial Number | rHR Pixel Scale (um) | Imaging Framerate (FPS) | Grating Velocity (mm/s) | Mass Flow Rate (ml/hr.) | Estimated Flow Exit Velocity (mm/s) | Reynolds Number | Allowable Shift per Frame (um) | Max Flow Shift per Frame (um) |
|---|---|---|---|---|---|---|---|---|
| 1 | 176 | 20 | 3.5 | 60 | 0.669 | 3.93 | 44 | 33.47 |
| 2 | 176 | 20 | 3.5 | 80 | 0.893 | 5.24 | 44 | 44.63 |
| 3 | 176 | 20 | 3.5 | 120 | 1.339 | 7.85 | 44 | 66.95 |
| 4 | 176 | 40.05 | 7.06 | 80 | 0.893 | 5.24 | 44 | 22.29 |
| 5 | 176 | 40.05 | 7.06 | 100 | 1.116 | 6.54 | 44 | 27.86 |
| 6 | 176 | 40.05 | 7.06 | 120 | 1.339 | 7.85 | 44 | 33.43 |
| 7 | 176 | 40.05 | 7.06 | 160 | 1.785 | 10.47 | 44 | 44.58 |

Supplemental Table S2: Trail Set Information and Timestamp for Figures

| Trial Number | Set Number | Grating Movement Direction | Frame in Set | Frame in Trial | Time (sec) | Estimated Flow Thickness (mm) |
|---|---|---|---|---|---|---|
| Trial 1 | Set 1 | Right | 1 | 0 | 0.00 | 2.54 |
| | Set 1 | Right | 401 | 800 | 20.00 | 3.12 |
| | Set 2 | Left | 1 | 130 | 3.25 | 2.61 |
| | Set 2 | Left | 401 | 800 | 20.00 | 3.62 |
| Trial 2 | Set 1 | Right | 1 | 0 | 0.00 | 5.07 |
| | Set 1 | Right | 401 | 800 | 20.00 | 2.32 |
| | Set 2 | Left | 1 | 129 | 3.23 | 3.12 |
| | Set 2 | Left | 401 | 800 | 20.00 | 2.97 |
| Trial 3 | Set 1 | Left | 1 | 0 | 0.00 | 3.19 |
| | Set 1 | Left | 401 | 800 | 20.00 | 3.62 |
| | Set 2 | Right | 1 | 150 | 3.75 | 3.62 |
| | Set 2 | Right | 401 | 800 | 20.00 | 3.84 |
| Trial 4 | Set 1 | Right | 1 | 0 | 0.00 | 3.70 |
| | Set 1 | Right | 401 | 400 | 9.99 | 3.62 |
| | Set 2 | Left | 1 | 70 | 1.75 | 3.70 |
| | Set 2 | Left | 401 | 400 | 9.99 | 3.91 |
| Trial 5 | Set 1 | Right | 1 | 0 | 0.00 | 3.84 |
| | Set 1 | Right | 401 | 400 | 9.99 | 3.70 |
| | Set 2 | Left | 1 | 83 | 2.07 | 3.77 |
| | Set 2 | Left | 401 | 400 | 9.99 | 3.77 |
| Trial 6 | Set 1 | Left | 1 | 0 | 0.00 | 3.55 |
| | Set 1 | Left | 401 | 400 | 9.99 | 3.19 |
| | Set 2 | Right | 1 | 70 | 1.75 | 3.41 |
| | Set 2 | Right | 401 | 400 | 9.99 | 3.33 |
| Trial 7 | Set 1 | Right | 1 | 0 | 0.00 | 3.26 |
| | Set 1 | Right | 401 | 400 | 9.99 | 3.04 |
| | Set 2 | Left | 1 | 74 | 1.85 | 3.48 |
| | Set 2 | Left | 401 | 400 | 9.99 | 3.55 |

**Flow Trial 1**

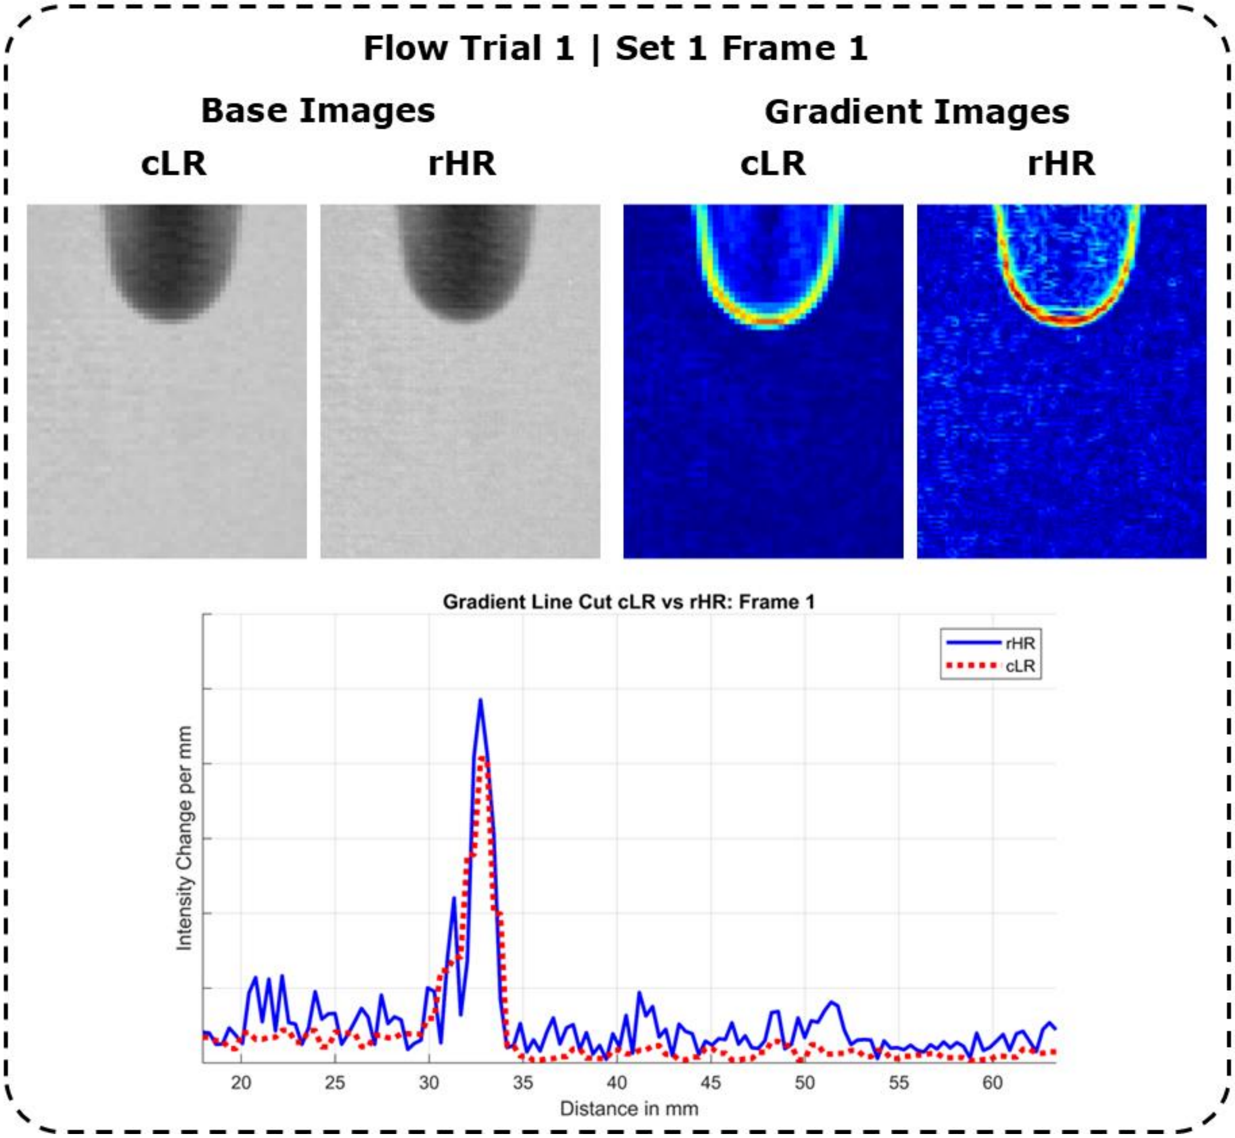


Supplemental Figure S1: Flow trial 1, set 1, frame 1 images, gradients, and gradient line cut.

Supplemental Figure S4 contains data from flow trial 1, set 1 frame 1 with an imaging frame rate of 20 FPS and a flow at 60 ml per hour. All images shown are cropped into the region of interest at the front of the flow. Captured low-resolution and reconstructed high-resolution images are shown along with their corresponding gradient. The gradient is normalized with respect to the pixel scale, 352 $\mu m$ for the cLR image and 176 $\mu m$ for the rHR image separately. We set the time for this initial frame to be 0 seconds. The gradient plot shows a vertical linecut of the center most column of pixels with the dashed red line denoting the cLR and the solid blue line denoting the rHR images. The x-axis shows the distance in mm from the exit of the nozzle. The y-axis is the intensity change normalized to the pixel scale with arbitrary units.

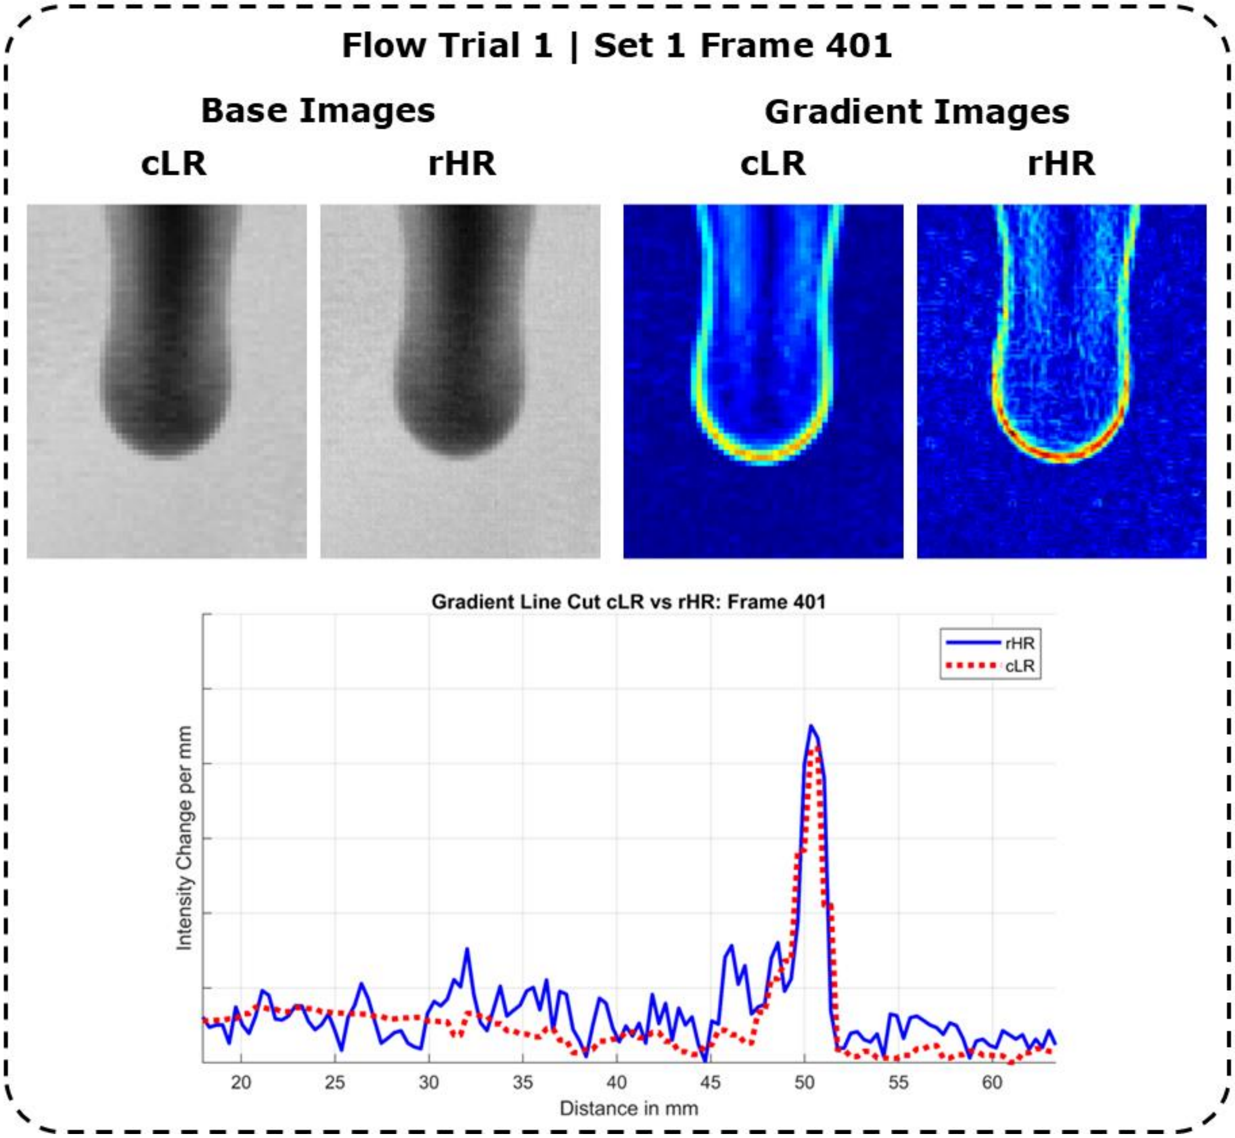


Supplemental Figure S2: Flow trial 1, set 1, frame 401 images, gradients, and gradient line cut.

Supplemental Figure S5 contains data from flow trial 1, set 1, frame 401 with an imaging frame rate of 20 FPS and a flow at 60 ml per hour. All images shown are cropped into the region of interest at the front of the flow. Captured low-resolution and reconstructed high-resolution images are shown along with their corresponding gradient. The gradient is normalized with respect to the pixel scale, 352 $\mu m$ for the cLR image and 176 $\mu m$ for the rHR image separately. This frame occurs 20 seconds after set 1, frame 1. The gradient plot shows a vertical linecut of the center most column of pixels with the dashed red line denoting the cLR and the solid blue line denoting the rHR images. The x-axis shows the distance in mm from the exit of the nozzle. The y-axis is the intensity change normalized to the pixel scale with arbitrary units.

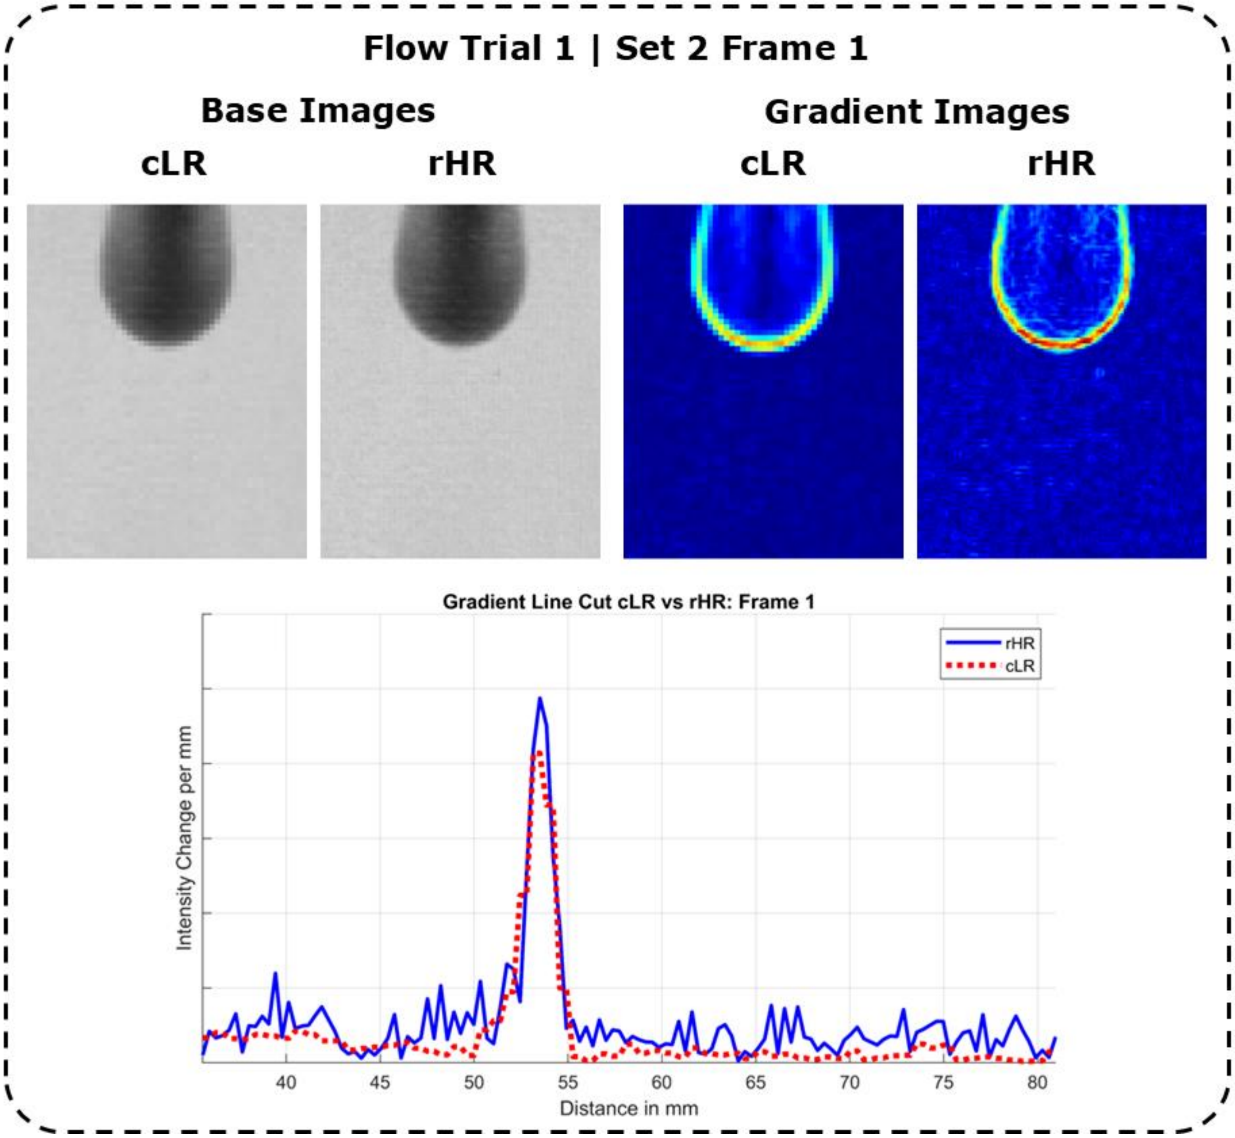


Supplemental Figure S3: Flow trial 1, set 2, frame 1 images, gradients, and gradient line cut.

Supplemental Figure S6 contains data from flow trial 1, set 2, frame 1 with an imaging frame rate of 20 FPS and a flow at 60 ml per hour. All images shown are cropped into the region of interest at the front of the flow. Captured low-resolution and reconstructed high-resolution images are shown along with their corresponding gradient. The gradient is normalized with respect to the pixel scale, 352 $\mu m$ for the cLR image and 176 $\mu m$ for the rHR image separately. This image occurs 23.25 seconds after set 1, frame 1. The gradient plot shows a vertical linecut of the center most column of pixels with the dashed red line denoting the cLR and the solid blue line denoting the rHR images. The x-axis shows the distance in mm from the exit of the nozzle. The y-axis is the intensity change normalized to the pixel scale with arbitrary units.

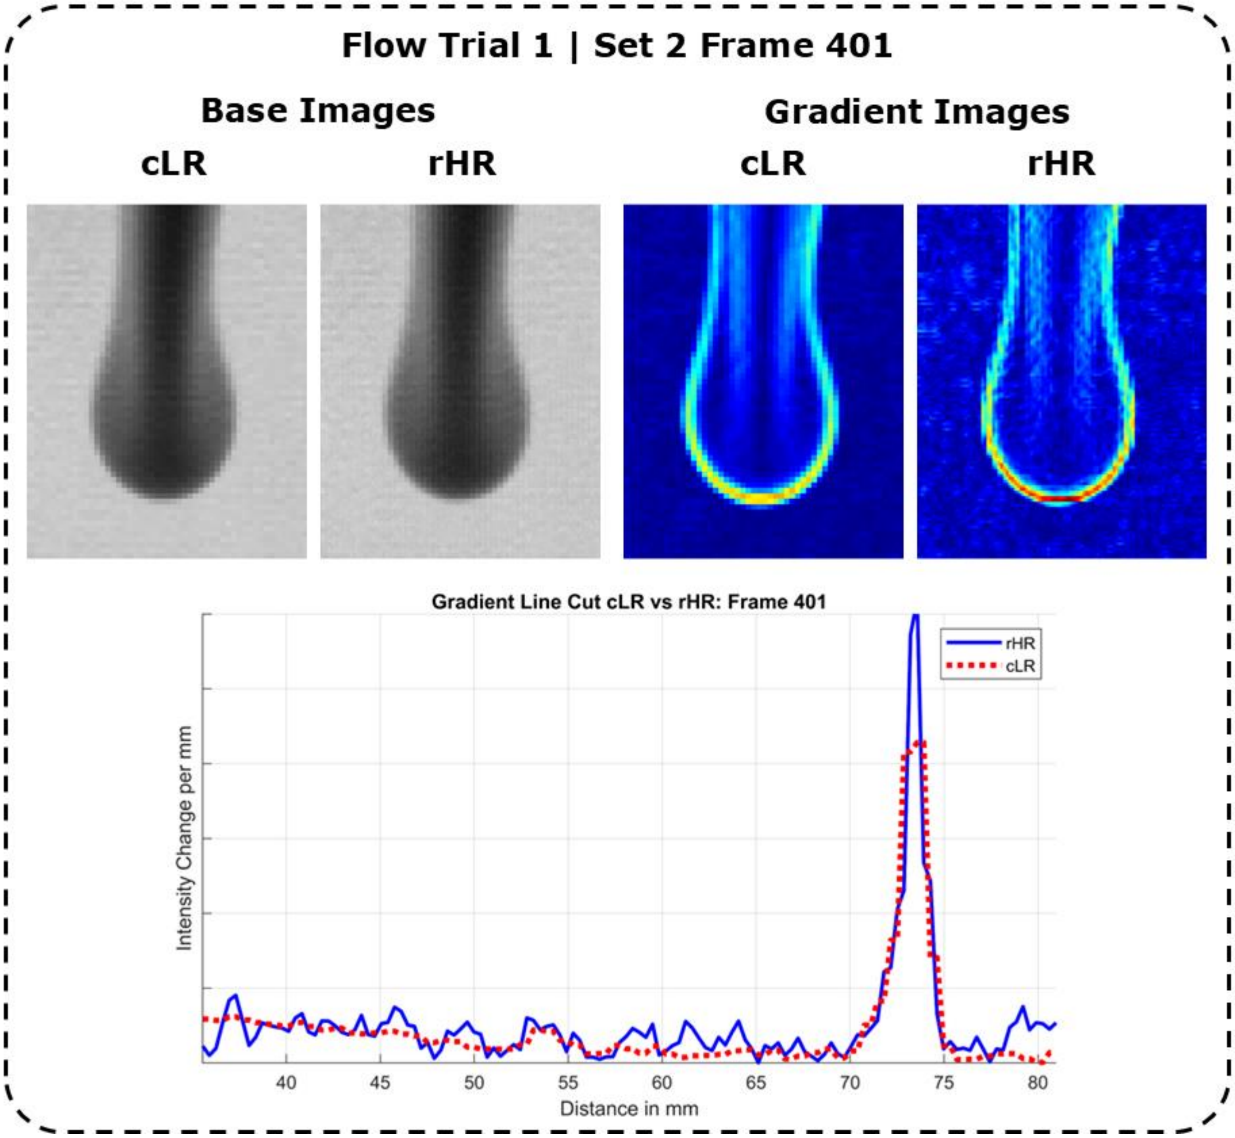


Supplemental Figure S4: Flow trial 1, set 2, frame 401 images, gradients, and gradient line cut.

Supplemental Figure S7 contains data from flow trial 1, set 2, frame 401 with an imaging frame rate of 20 FPS and a flow at 60 ml per hour. All images shown are cropped into the region of interest at the front of the flow. Captured low-resolution and reconstructed high-resolution images are shown along with their corresponding gradient. The gradient is normalized with respect to the pixel scale, 352 $\mu m$ for the cLR image and 176 $\mu m$ for the rHR image separately. This image occurs 43.25 seconds after set 1, frame 1. The gradient plot shows a vertical linecut of the center most column of pixels with the dashed red line denoting the cLR and the solid blue line denoting the rHR images. The x-axis shows the distance in mm from the exit of the nozzle. The y-axis is the intensity change normalized to the pixel scale with arbitrary units.

**Flow Trial 2**

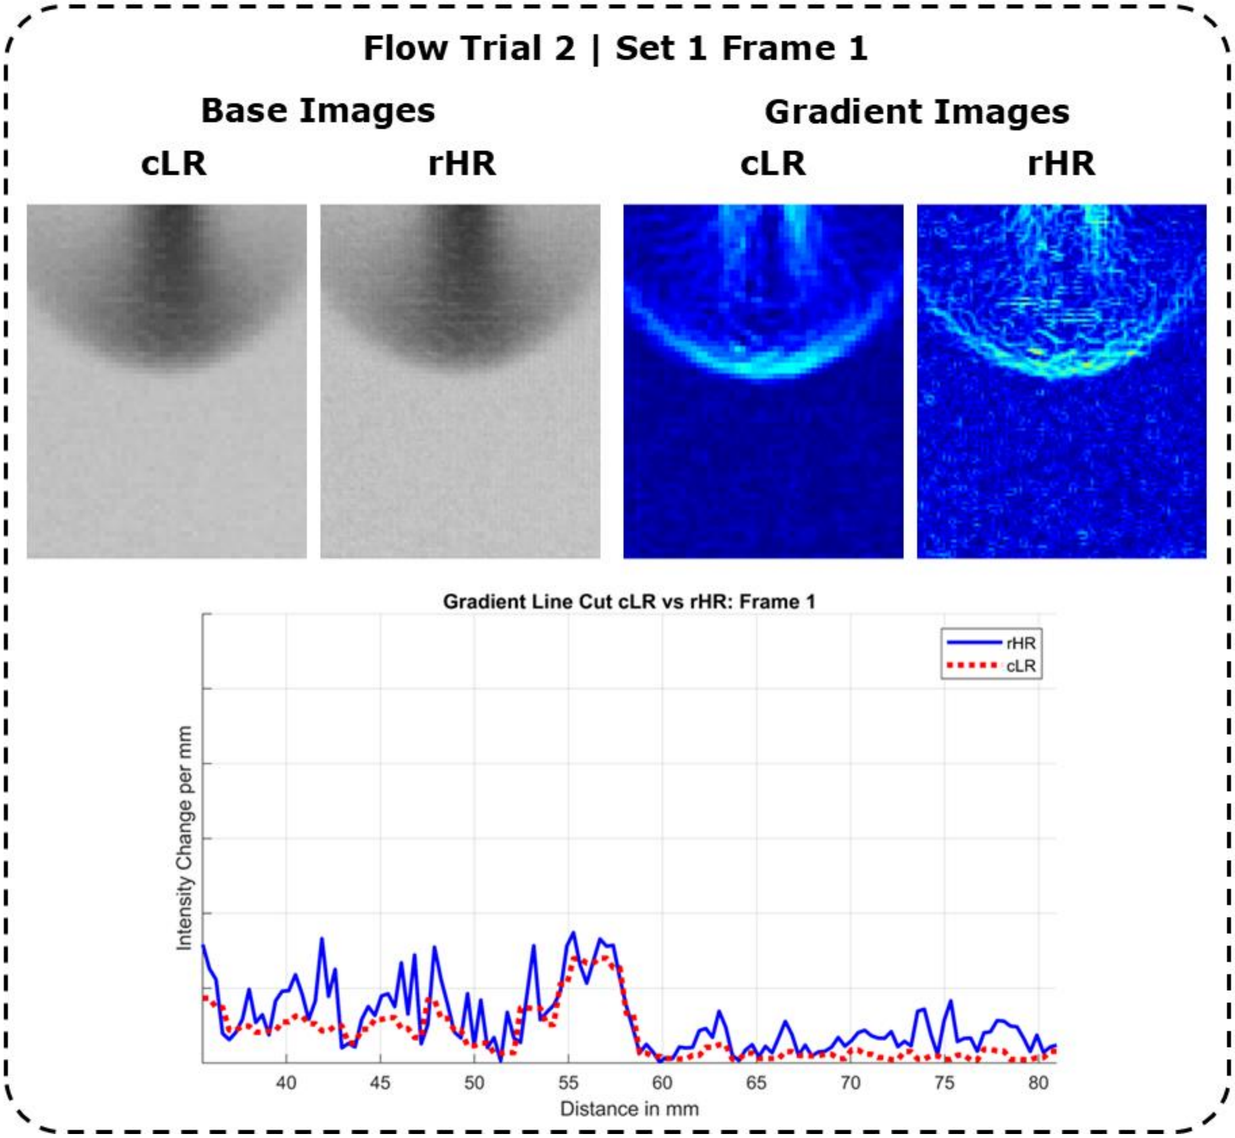


Supplemental Figure S5: Flow trial 2, set 1, frame 1 images, gradients, and gradient line cut.

Supplemental Figure S8 contains data from flow trial 2, set 1 frame 1 with an imaging frame rate of 20 FPS and a flow at 80 ml per hour. All images shown are cropped into the region of interest at the front of the flow. Captured low-resolution and reconstructed high-resolution images are shown along with their corresponding gradient. The gradient is normalized with respect to the pixel scale, 352 $\mu m$ for the cLR image and 176 $\mu m$ for the rHR image separately. We set the time for this initial frame to be 0 seconds. The gradient plot shows a vertical linecut of the center most column of pixels with the dashed red line denoting the cLR and the solid blue line denoting the rHR images. The x-axis shows the distance in mm from the exit of the nozzle. The y-axis is the intensity change normalized to the pixel scale with arbitrary units.

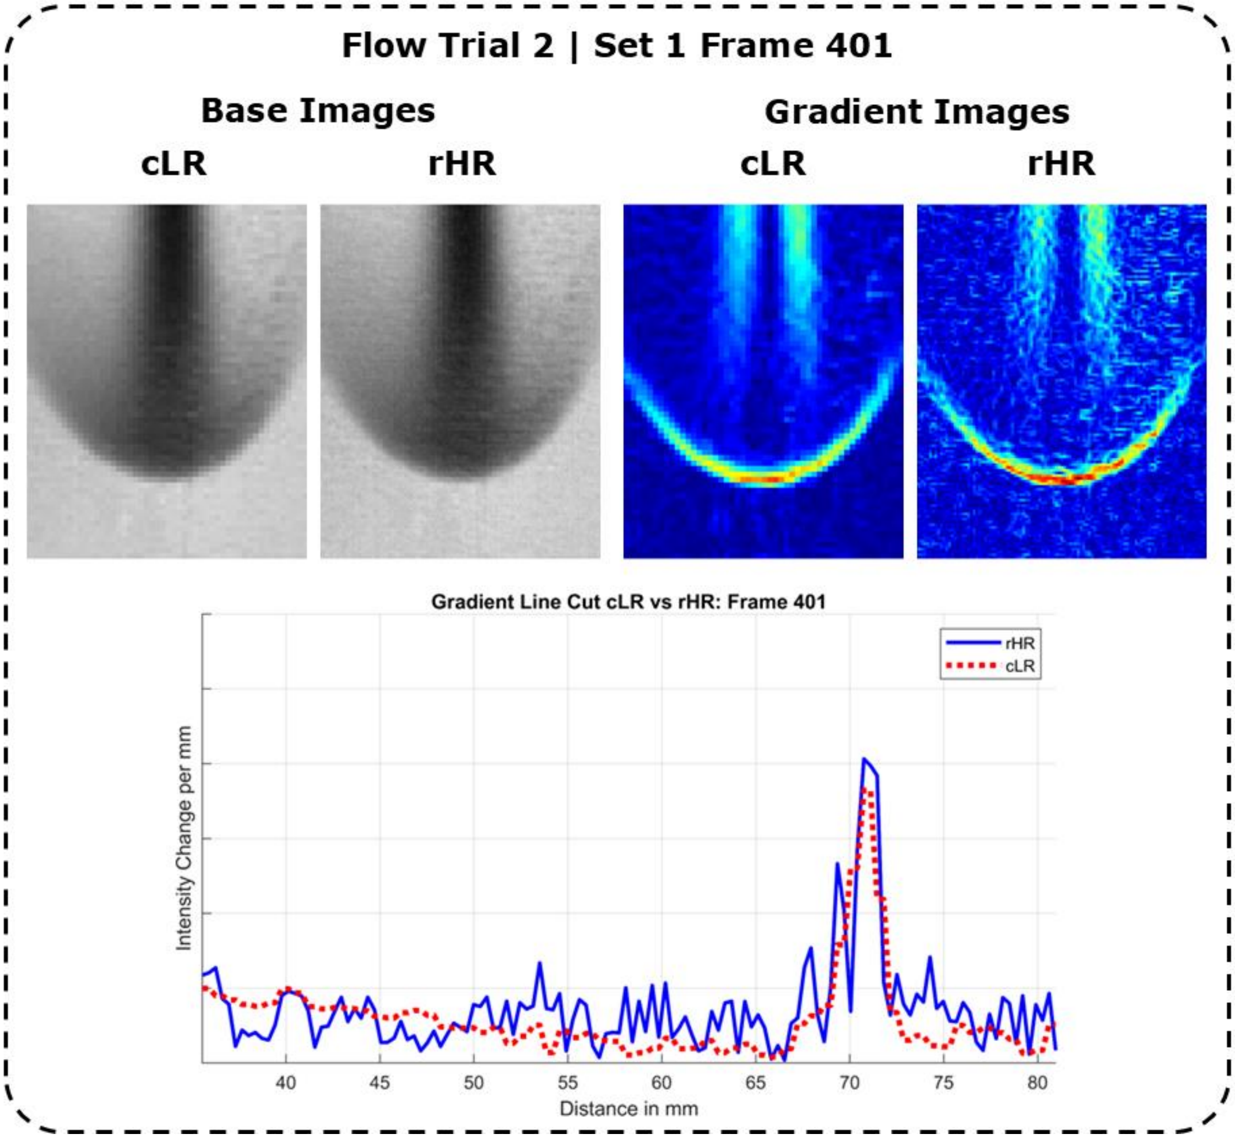


Supplemental Figure S6: Flow trial 2, set 1, frame 401 images, gradients, and gradient line cut.

Supplemental Figure S9 contains data from flow trial 2, set 1, frame 401 with an imaging frame rate of 20 FPS and a flow at 80 ml per hour. All images shown are cropped into the region of interest at the front of the flow. Captured low-resolution and reconstructed high-resolution images are shown along with their corresponding gradient. The gradient is normalized with respect to the pixel scale, 352 $\mu m$ for the cLR image and 176 $\mu m$ for the rHR image separately. This frame occurs 20 seconds after set 1, frame 1. The gradient plot shows a vertical linecut of the center most column of pixels with the dashed red line denoting the cLR and the solid blue line denoting the rHR images. The x-axis shows the distance in mm from the exit of the nozzle. The y-axis is the intensity change normalized to the pixel scale with arbitrary units.

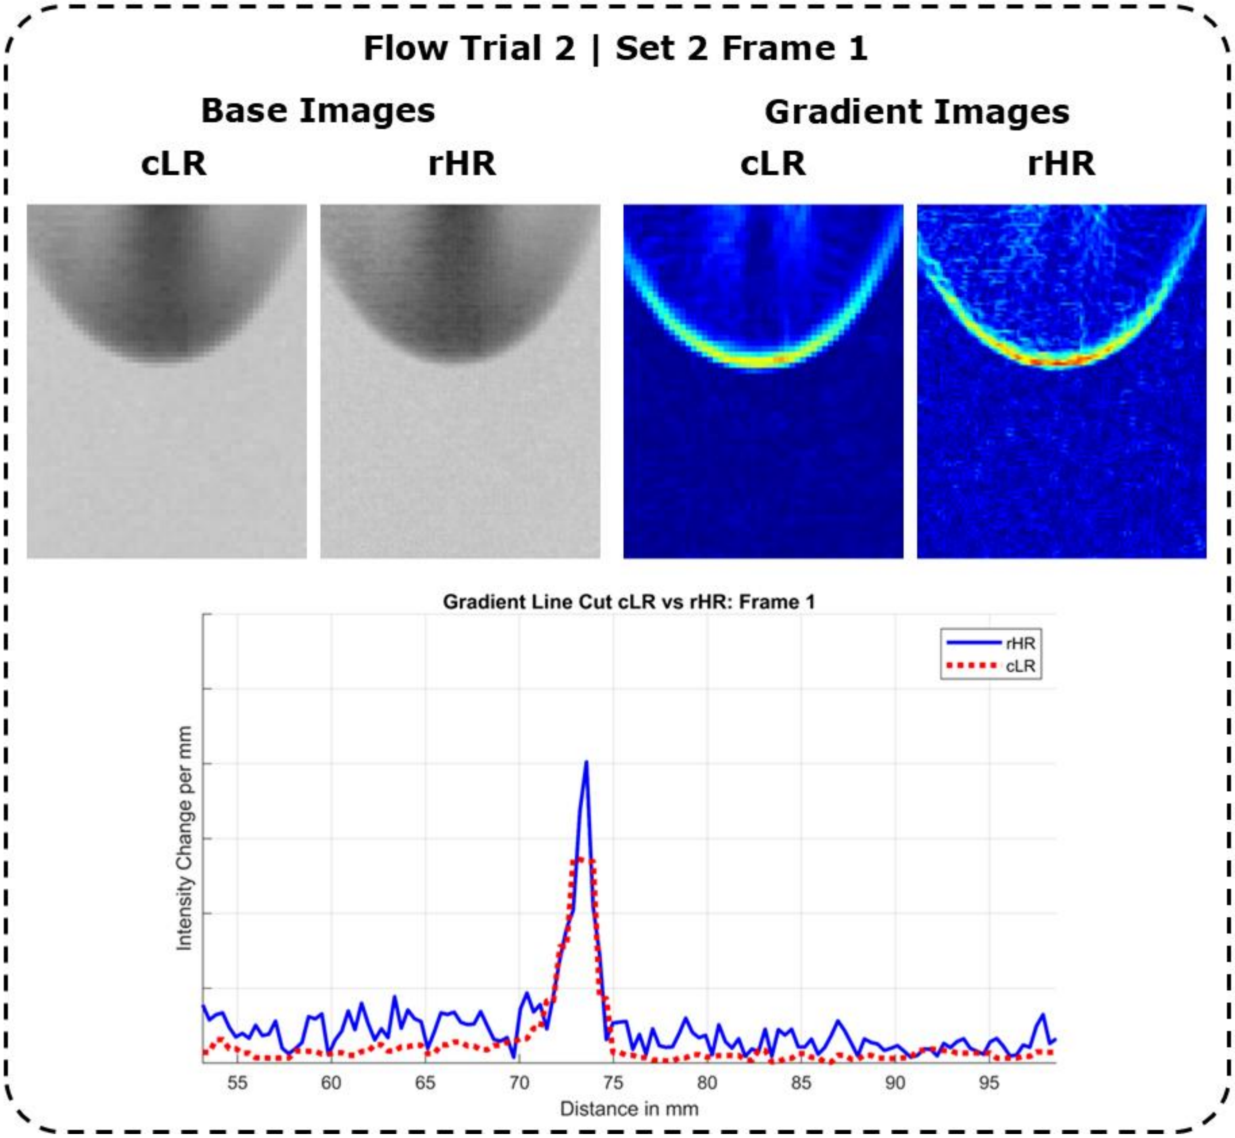


Supplemental Figure S7: Flow trial 2, set 2, frame 1 images, gradients, and gradient line cut.

Supplemental Figure S10 contains data from flow trial 2, set 2, frame 1 with an imaging frame rate of 20 FPS and a flow at 80 ml per hour. All images shown are cropped into the region of interest at the front of the flow. Captured low-resolution and reconstructed high-resolution images are shown along with their corresponding gradient. The gradient is normalized with respect to the pixel scale, 352 $\mu m$ for the cLR image and 176 $\mu m$ for the rHR image separately. This image occurs 23.23 seconds after set 1, frame 1. The gradient plot shows a vertical linecut of the center most column of pixels with the dashed red line denoting the cLR and the solid blue line denoting the rHR images. The x-axis shows the distance in mm from the exit of the nozzle. The y-axis is the intensity change normalized to the pixel scale with arbitrary units.

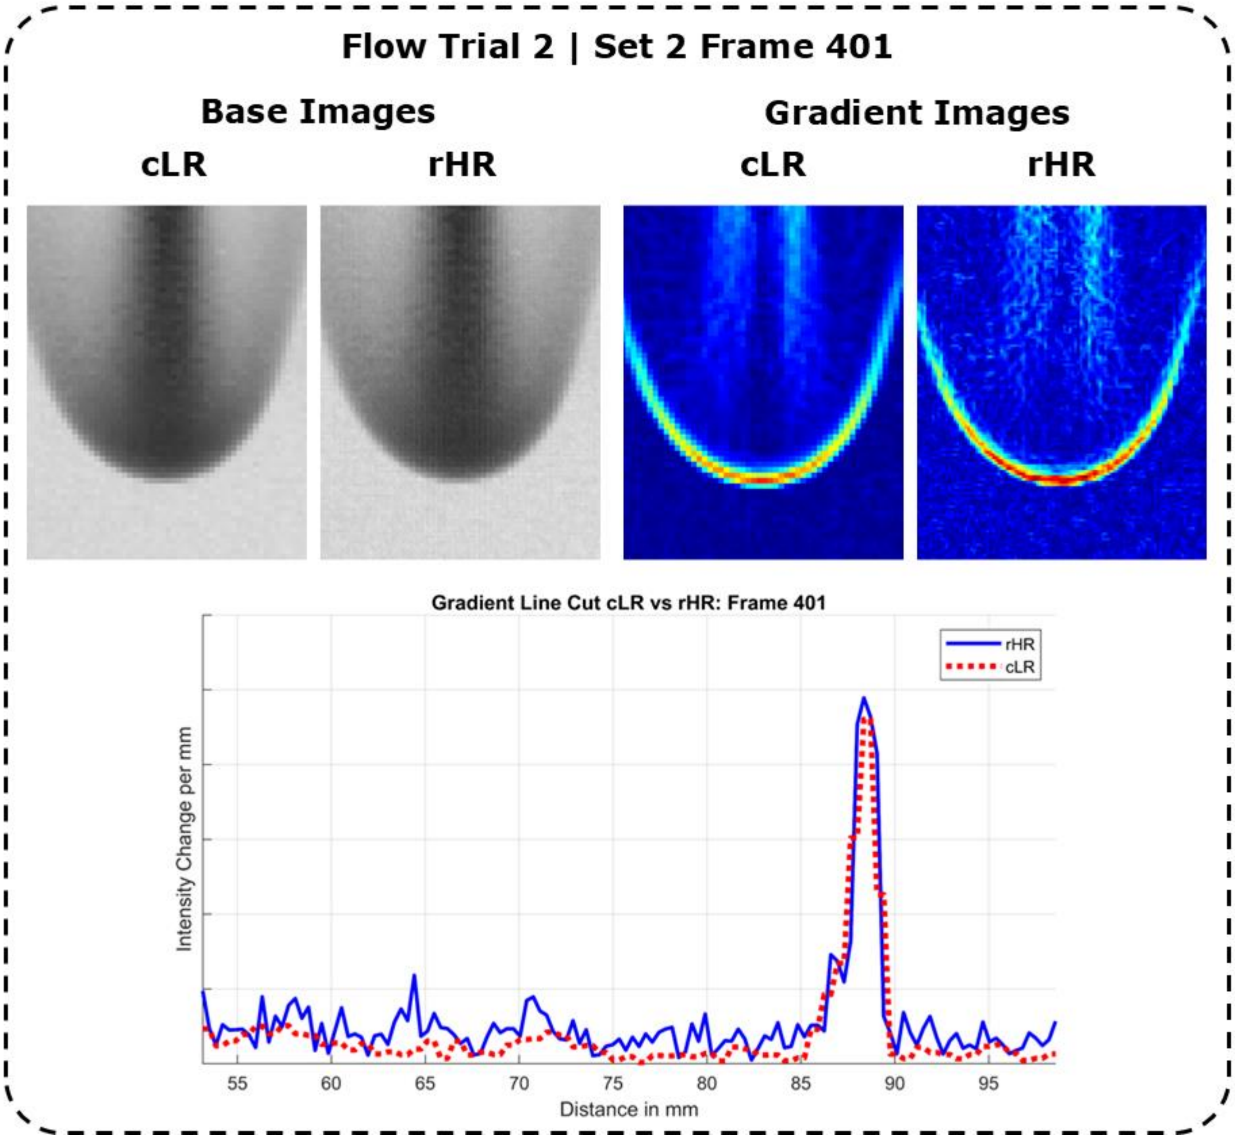


Supplemental Figure S8: Flow trial 2, set 2, frame 401 images, gradients, and gradient line cut.

Supplemental Figure S11 contains data from flow trial 2, set 2, frame 401 with an imaging frame rate of 20 FPS and a flow at 80 ml per hour. All images shown are cropped into the region of interest at the front of the flow. Captured low-resolution and reconstructed high-resolution images are shown along with their corresponding gradient. The gradient is normalized with respect to the pixel scale, 352 $\mu m$ for the cLR image and 176 $\mu m$ for the rHR image separately. This image occurs 43.23 seconds after set 1, frame 1. The gradient plot shows a vertical linecut of the center most column of pixels with the dashed red line denoting the cLR and the solid blue line denoting the rHR images. The x-axis shows the distance in mm from the exit of the nozzle. The y-axis is the intensity change normalized to the pixel scale with arbitrary units.

**Flow Trial 3**

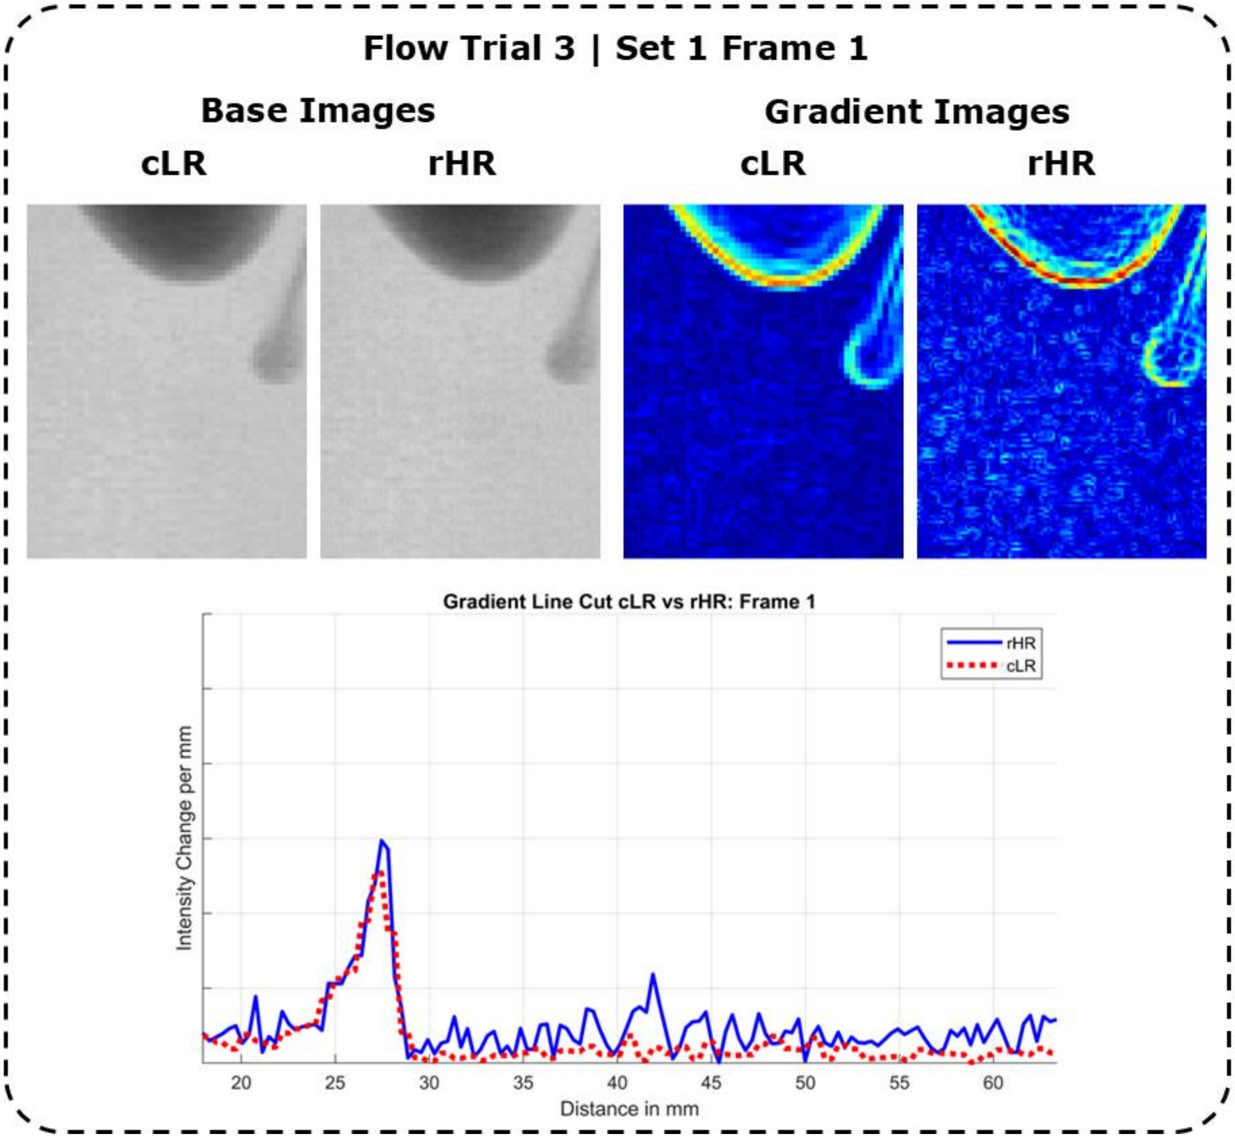


Supplemental Figure S9: Flow trial 3, set 1, frame 1 images, gradients, and gradient line cut.

Supplemental Figure S12 contains data from flow trial 3, set 1 frame 1 with an imaging frame rate of 20 FPS and a flow at 120 ml per hour. All images shown are cropped into the region of interest at the front of the flow. Captured low-resolution and reconstructed high-resolution images are shown along with their corresponding gradient. The gradient is normalized with respect to the pixel scale, 352 $\mu m$ for the cLR image and 176 $\mu m$ for the rHR image separately. We set the time for this initial frame to be 0 seconds. The gradient plot shows a vertical linecut of the center most column of pixels with the dashed red line denoting the cLR and the solid blue line denoting the rHR images. The x-axis shows the distance in mm from the exit of the nozzle. The y-axis is the intensity change normalized to the pixel scale with arbitrary units.

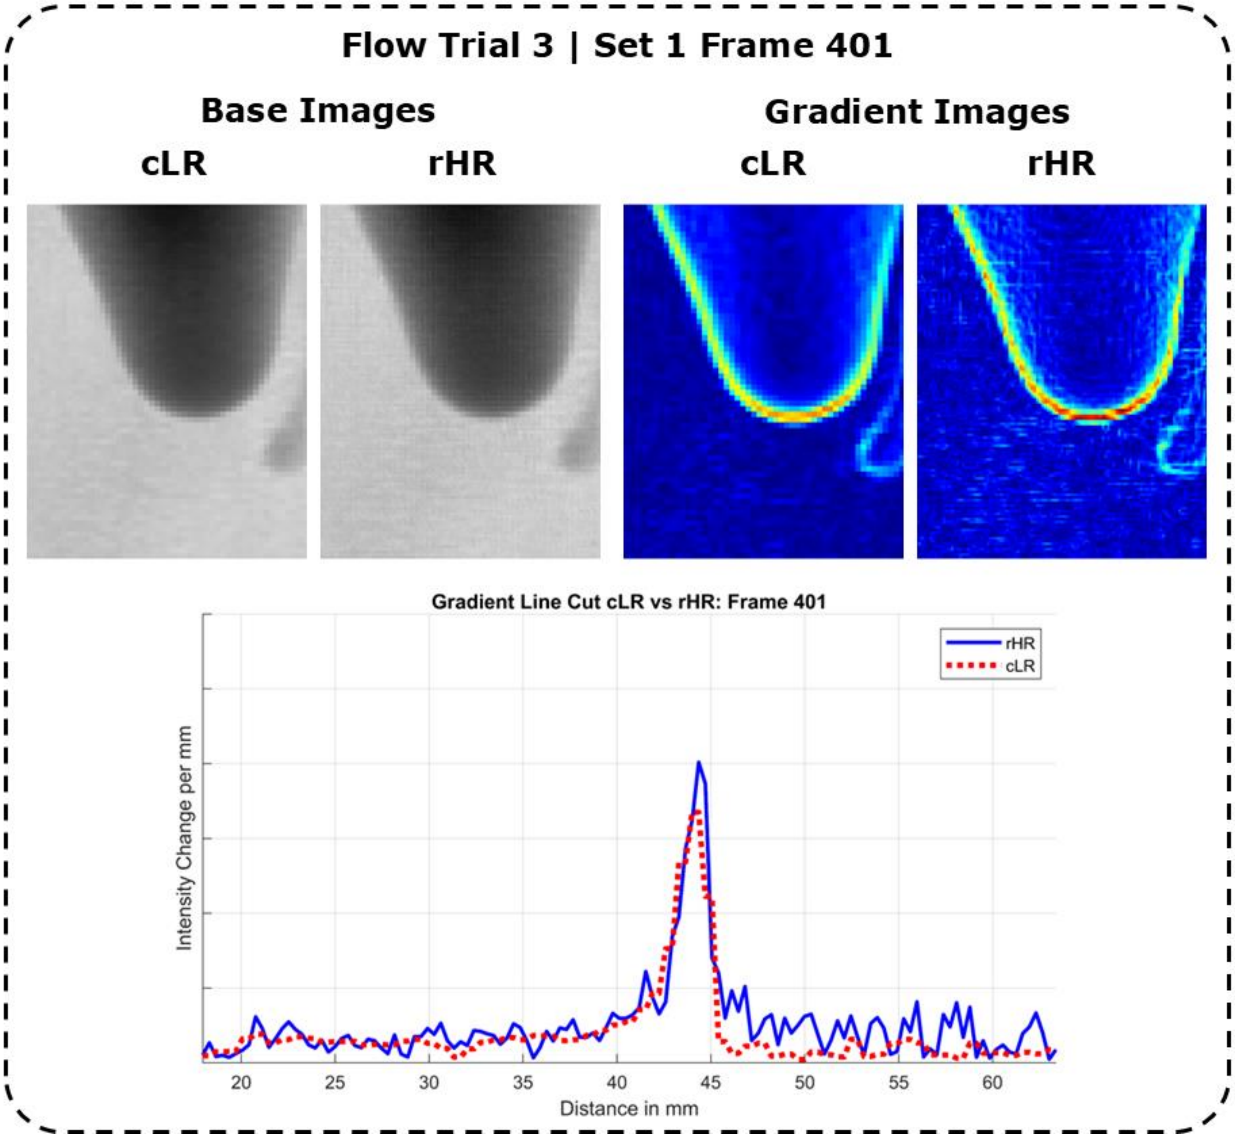


Supplemental Figure S10: Flow trial 3, set 1, frame 401 images, gradients, and gradient line cut.

Supplemental Figure S13 contains data from flow trial 3, set 1, frame 401 with an imaging frame rate of 20 FPS and a flow at 120 ml per hour. All images shown are cropped into the region of interest at the front of the flow. Captured low-resolution and reconstructed high-resolution images are shown along with their corresponding gradient. The gradient is normalized with respect to the pixel scale, 352 $\mu m$ for the cLR image and 176 $\mu m$ for the rHR image separately. This frame occurs 20 seconds after set 1, frame 1. The gradient plot shows a vertical linecut of the center most column of pixels with the dashed red line denoting the cLR and the solid blue line denoting the rHR images. The x-axis shows the distance in mm from the exit of the nozzle. The y-axis is the intensity change normalized to the pixel scale with arbitrary units.

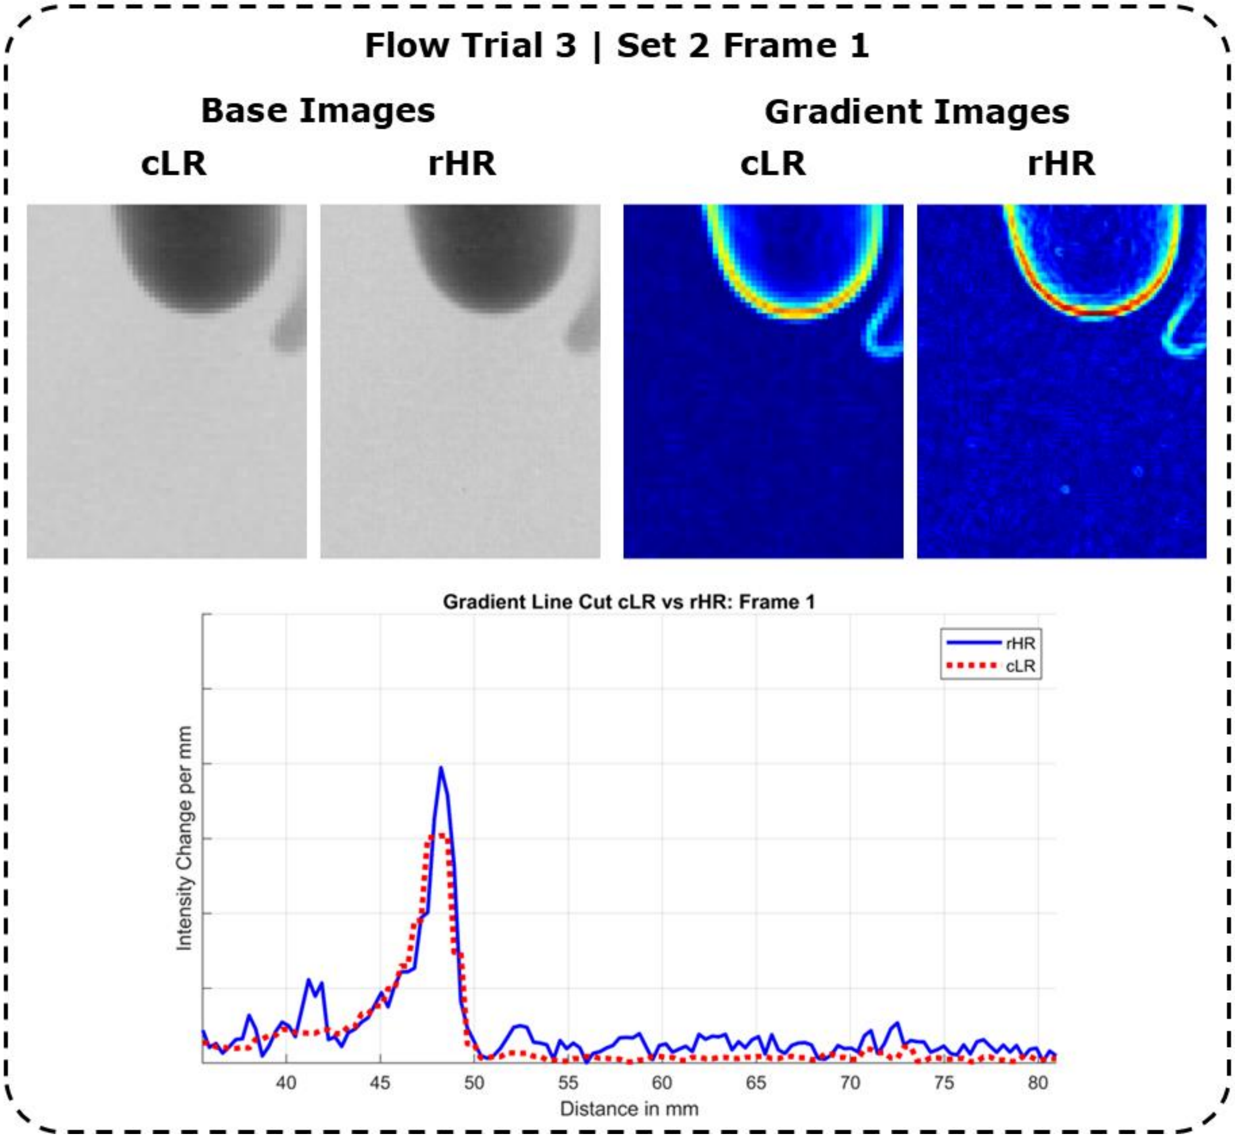


Supplemental Figure S11: Flow trial 3, set 2, frame 1 images, gradients, and gradient line cut.

Supplemental Figure S14 contains data from flow trial 3, set 2, frame 1 with an imaging frame rate of 20 FPS and a flow at 120 ml per hour. All images shown are cropped into the region of interest at the front of the flow. Captured low-resolution and reconstructed high-resolution images are shown along with their corresponding gradient. The gradient is normalized with respect to the pixel scale, 352 $\mu m$ for the cLR image and 176 $\mu m$ for the rHR image separately. This image occurs 23.75 seconds after set 1, frame 1. The gradient plot shows a vertical linecut of the center most column of pixels with the dashed red line denoting the cLR and the solid blue line denoting the rHR images. The x-axis shows the distance in mm from the exit of the nozzle. The y-axis is the intensity change normalized to the pixel scale with arbitrary units.

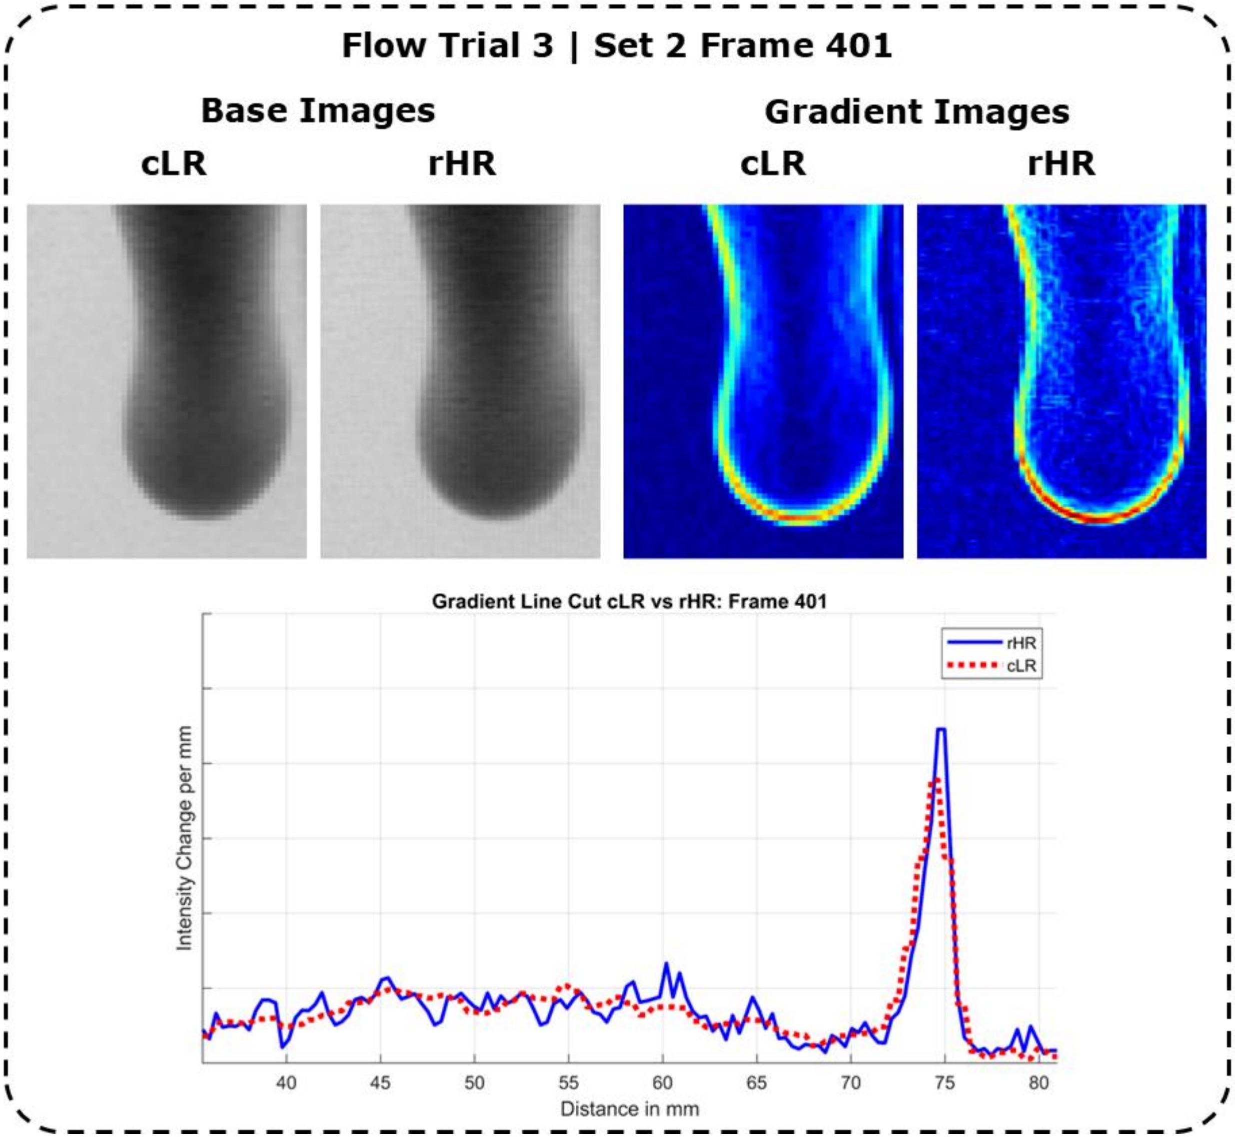


Supplemental Figure S12: Flow trial 3, set 2, frame 401 images, gradients, and gradient line cut.

Supplemental Figure S15 contains data from flow trial 3, set 2, frame 401 with an imaging frame rate of 20 FPS and a flow at 120 ml per hour. All images shown are cropped into the region of interest at the front of the flow. Captured low-resolution and reconstructed high-resolution images are shown along with their corresponding gradient. The gradient is normalized with respect to the pixel scale, 352 $\mu m$ for the cLR image and 176 $\mu m$ for the rHR image separately. This image occurs 43.75 seconds after set 1, frame 1. The gradient plot shows a vertical linecut of the center most column of pixels with the dashed red line denoting the cLR and the solid blue line denoting the rHR images. The x-axis shows the distance in mm from the exit of the nozzle. The y-axis is the intensity change normalized to the pixel scale with arbitrary units.

**Flow Trial 4**

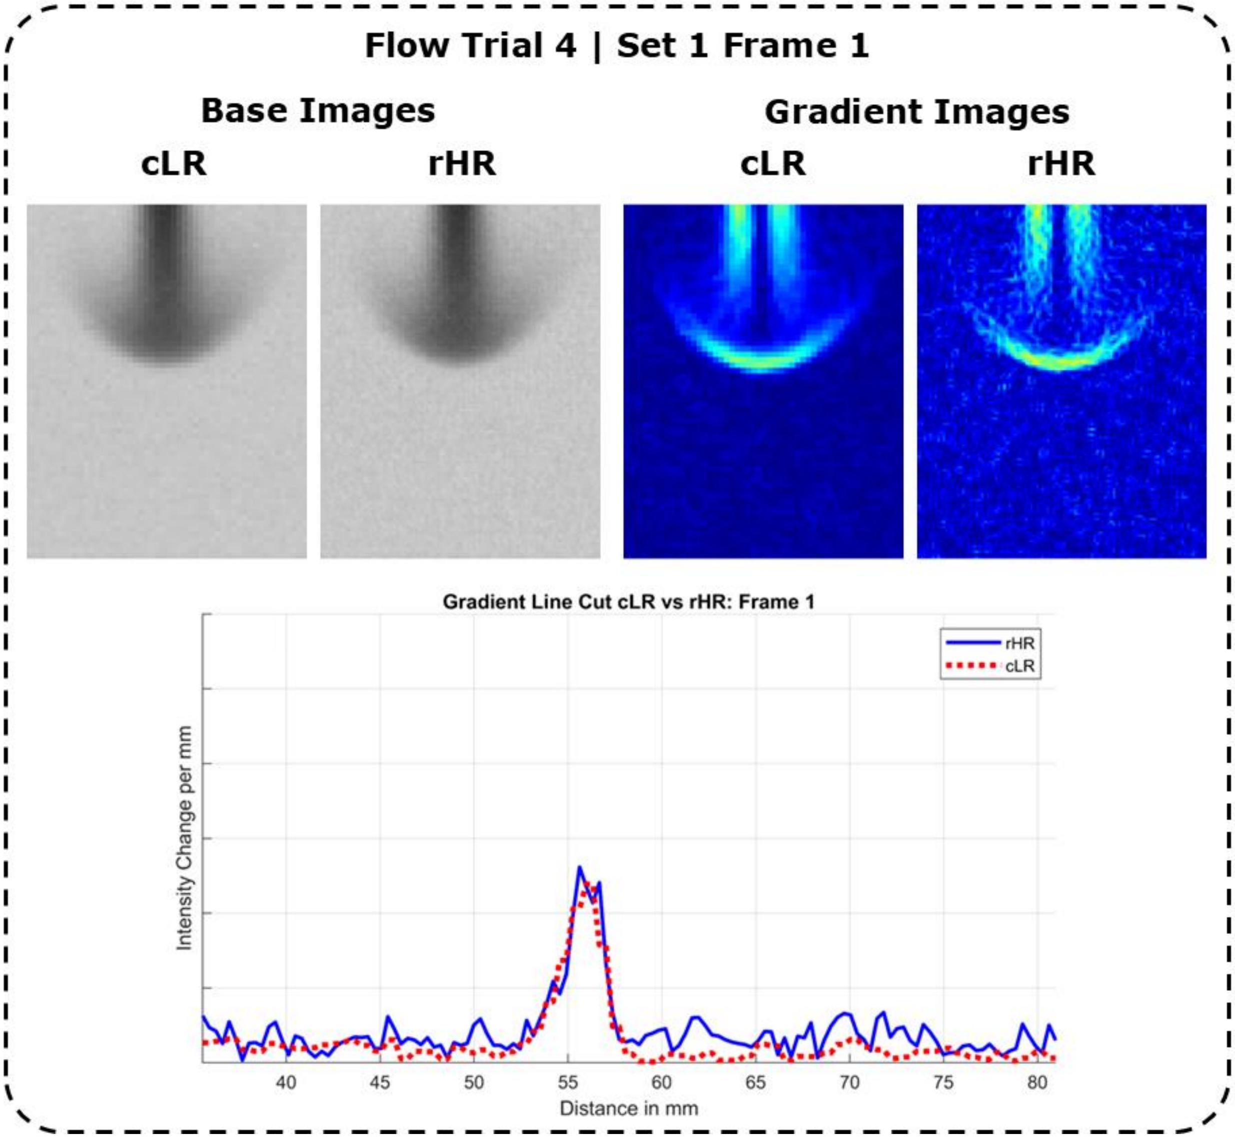


Supplemental Figure S13: Flow trial 4, set 1, frame 1 images, gradients, and gradient line cut.

Supplemental Figure S16 contains data from flow trial 4, set 1 frame 1 with an imaging frame rate of 40.05 FPS and a flow at 60 ml per hour. All images shown are cropped into the region of interest at the front of the flow. Captured low-resolution and reconstructed high-resolution images are shown along with their corresponding gradient. The gradient is normalized with respect to the pixel scale, 352 $\mu m$ for the cLR image and 176 $\mu m$ for the rHR image separately. We set the time for this initial frame to be 0 seconds. The gradient plot shows a vertical linecut of the center most column of pixels with the dashed red line denoting the cLR and the solid blue line denoting the rHR images. The x-axis shows the distance in mm from the exit of the nozzle. The y-axis is the intensity change normalized to the pixel scale with arbitrary units.

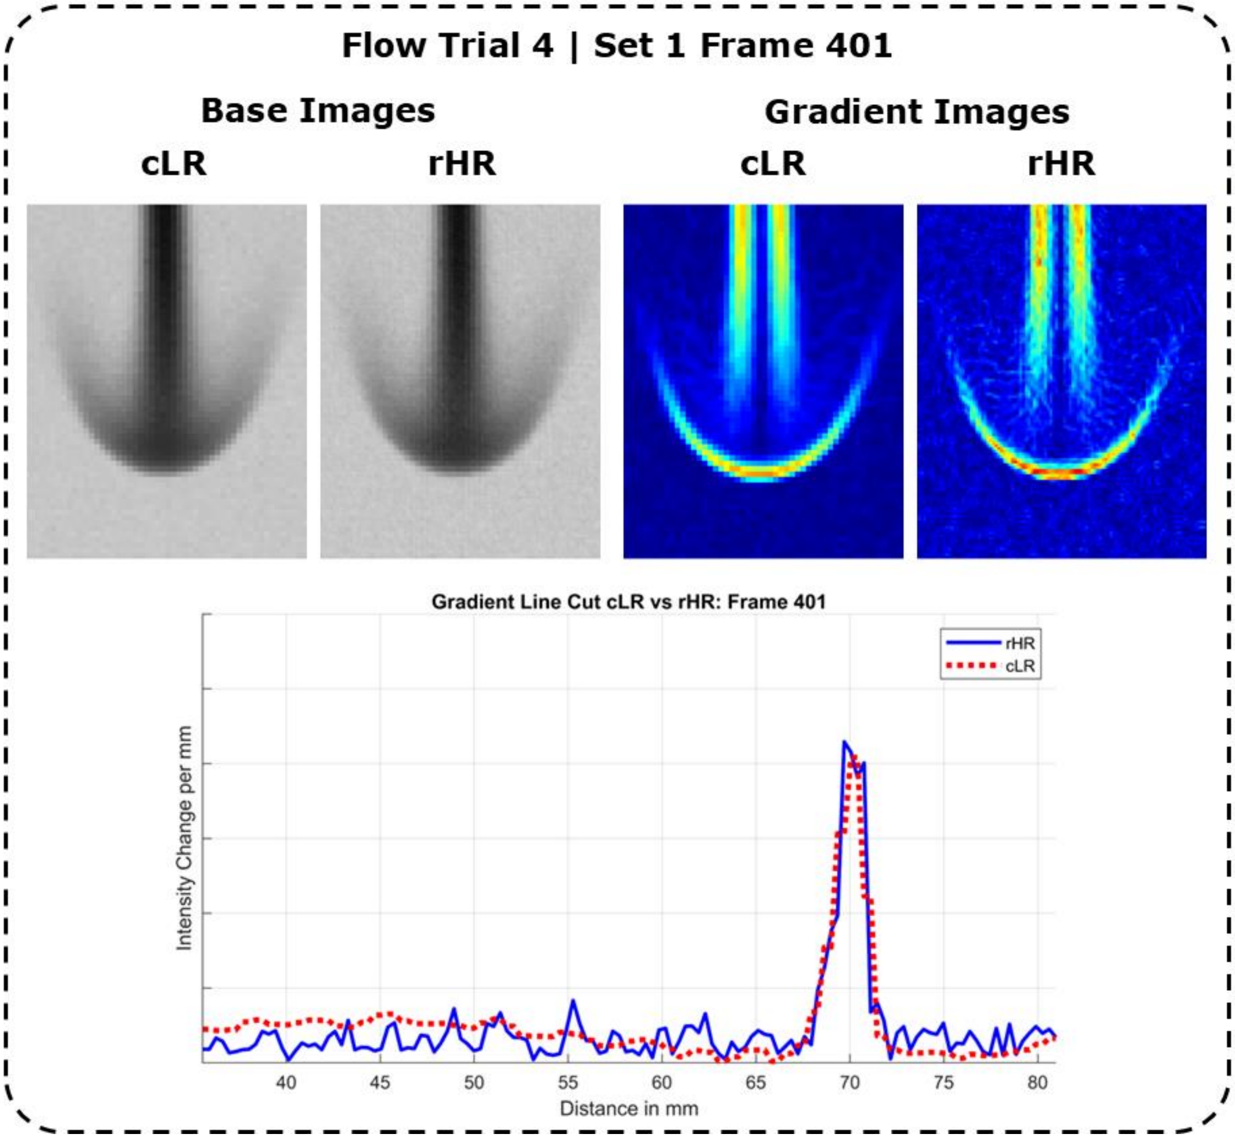


Supplemental Figure S14: Flow trial 4, set 1, frame 401 images, gradients, and gradient line cut.

Supplemental Figure S17 contains data from flow trial 4, set 1, frame 401 with an imaging frame rate of 40.05 FPS and a flow at 60 ml per hour. All images shown are cropped into the region of interest at the front of the flow. Captured low-resolution and reconstructed high-resolution images are shown along with their corresponding gradient. The gradient is normalized with respect to the pixel scale, 352 $\mu m$ for the cLR image and 176 $\mu m$ for the rHR image separately. This frame occurs 9.99 seconds after set 1, frame 1. The gradient plot shows a vertical linecut of the center most column of pixels with the dashed red line denoting the cLR and the solid blue line denoting the rHR images. The x-axis shows the distance in mm from the exit of the nozzle. The y-axis is the intensity change normalized to the pixel scale with arbitrary units.

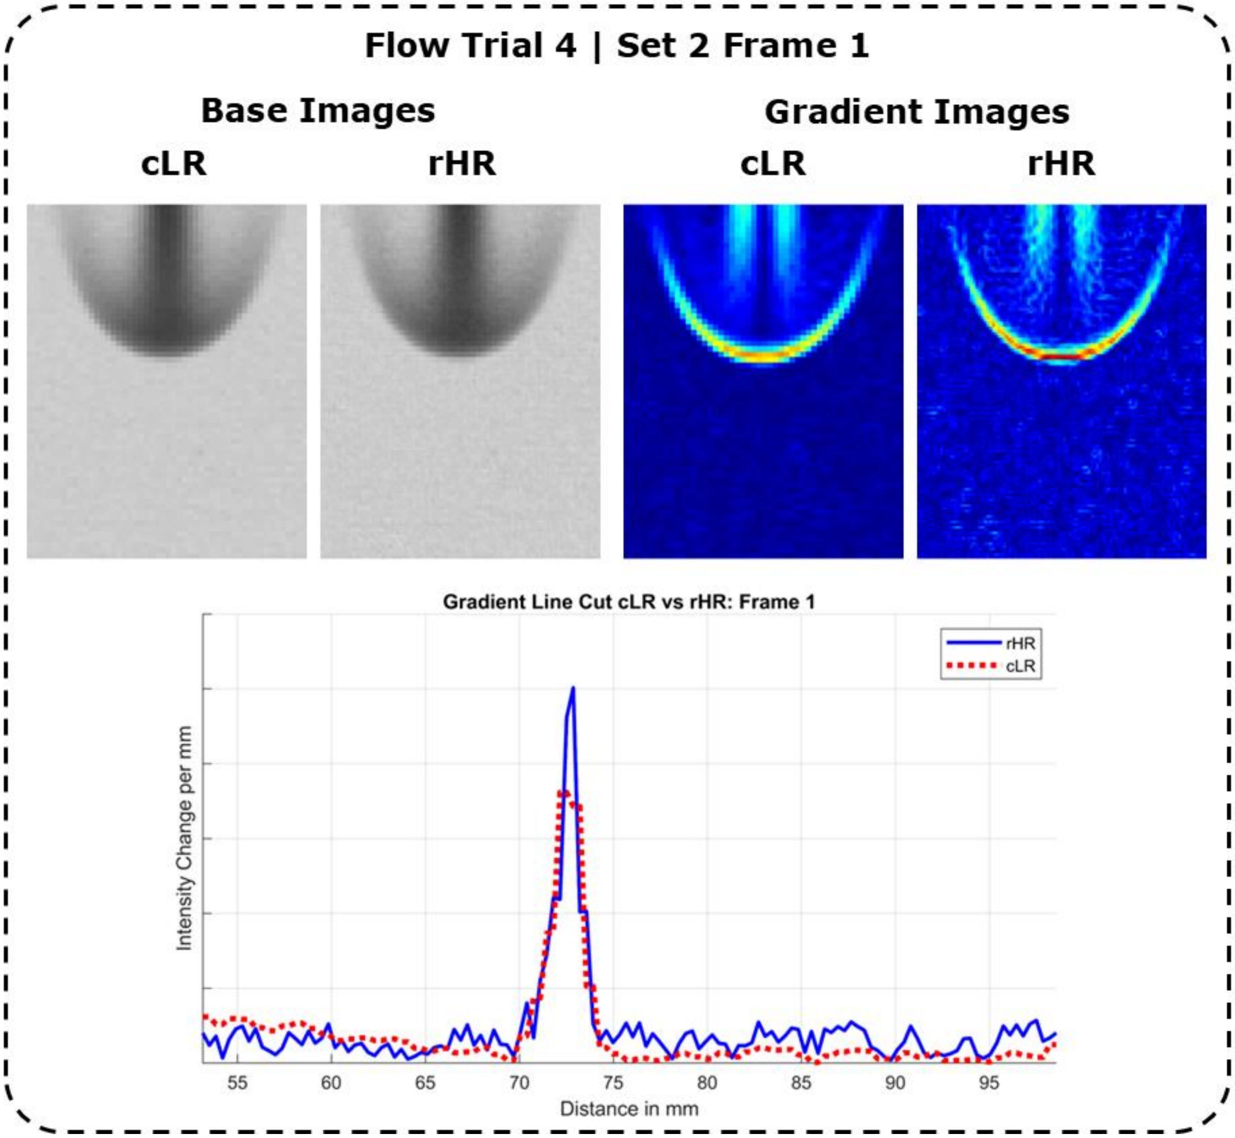


Supplemental Figure S15: Flow trial 4, set 2, frame 1 images, gradients, and gradient line cut.

Supplemental Figure S18 contains data from flow trial 4, set 2, frame 1 with an imaging frame rate of 40.05 FPS and a flow at 60 ml per hour. All images shown are cropped into the region of interest at the front of the flow. Captured low-resolution and reconstructed high-resolution images are shown along with their corresponding gradient. The gradient is normalized with respect to the pixel scale, 352 $\mu m$ for the cLR image and 176 $\mu m$ for the rHR image separately. This image occurs 11.74 seconds after set 1, frame 1. The gradient plot shows a vertical linecut of the center most column of pixels with the dashed red line denoting the cLR and the solid blue line denoting the rHR images. The x-axis shows the distance in mm from the exit of the nozzle. The y-axis is the intensity change normalized to the pixel scale with arbitrary units.

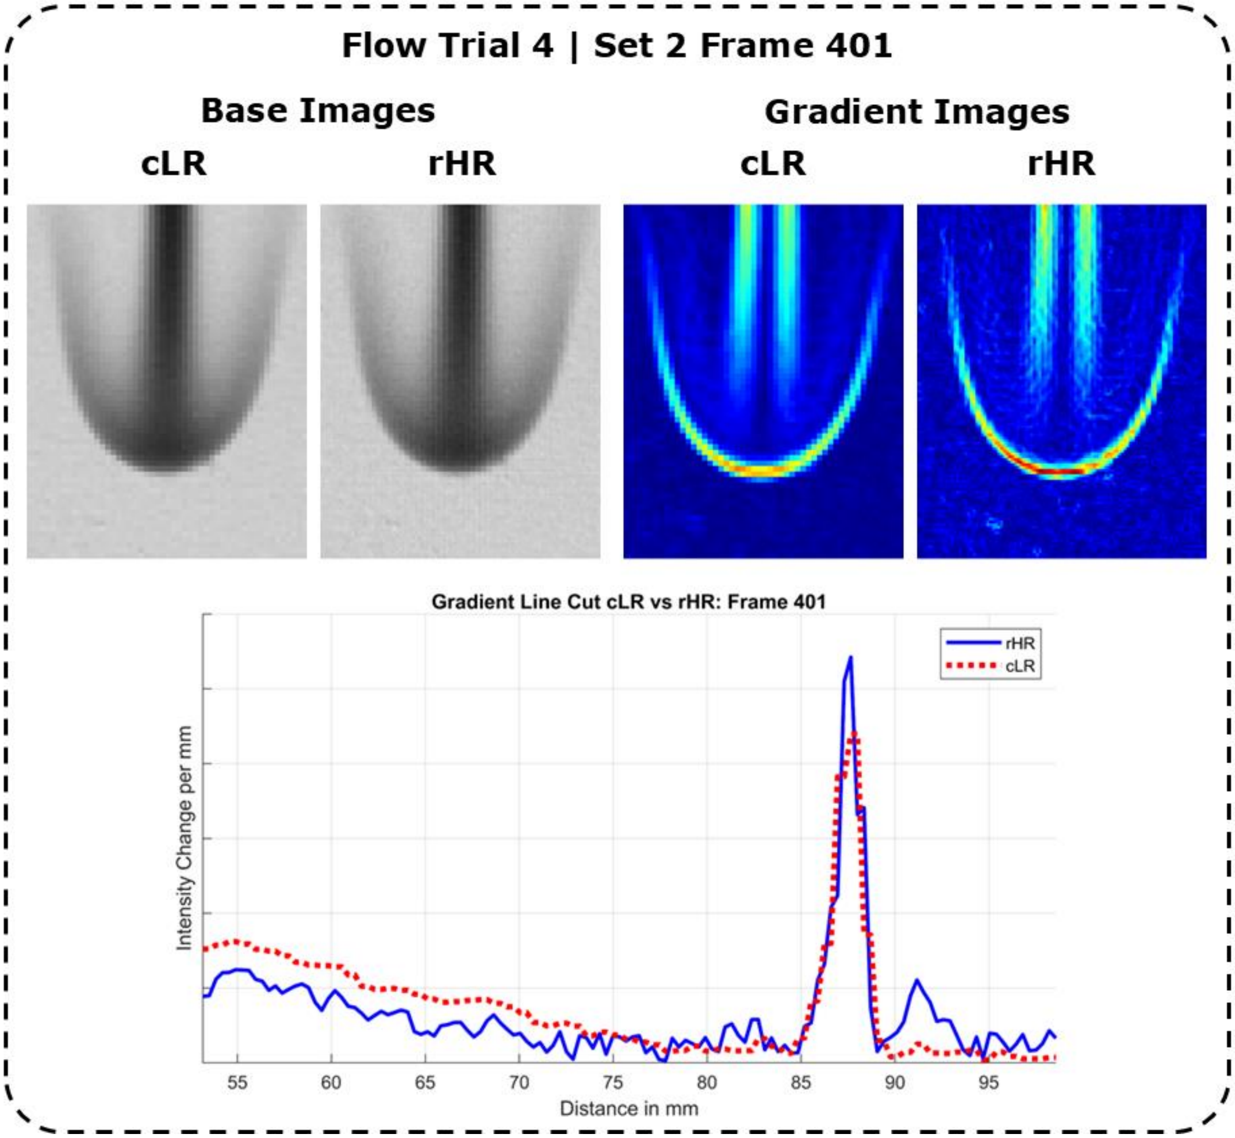


Supplemental Figure S16: Flow trial 4, set 2, frame 401 images, gradients, and gradient line cut.

Supplemental Figure S19 contains data from flow trial 4, set 2, frame 401 with an imaging frame rate of 40.05 FPS and a flow at 60 ml per hour. All images shown are cropped into the region of interest at the front of the flow. Captured low-resolution and reconstructed high-resolution images are shown along with their corresponding gradient. The gradient is normalized with respect to the pixel scale, 352 $\mu m$ for the cLR image and 176 $\mu m$ for the rHR image separately. This image occurs 21.72 seconds after set 1, frame 1. The gradient plot shows a vertical linecut of the center most column of pixels with the dashed red line denoting the cLR and the solid blue line denoting the rHR images. The x-axis shows the distance in mm from the exit of the nozzle. The y-axis is the intensity change normalized to the pixel scale with arbitrary units.

**Flow Trial 5**

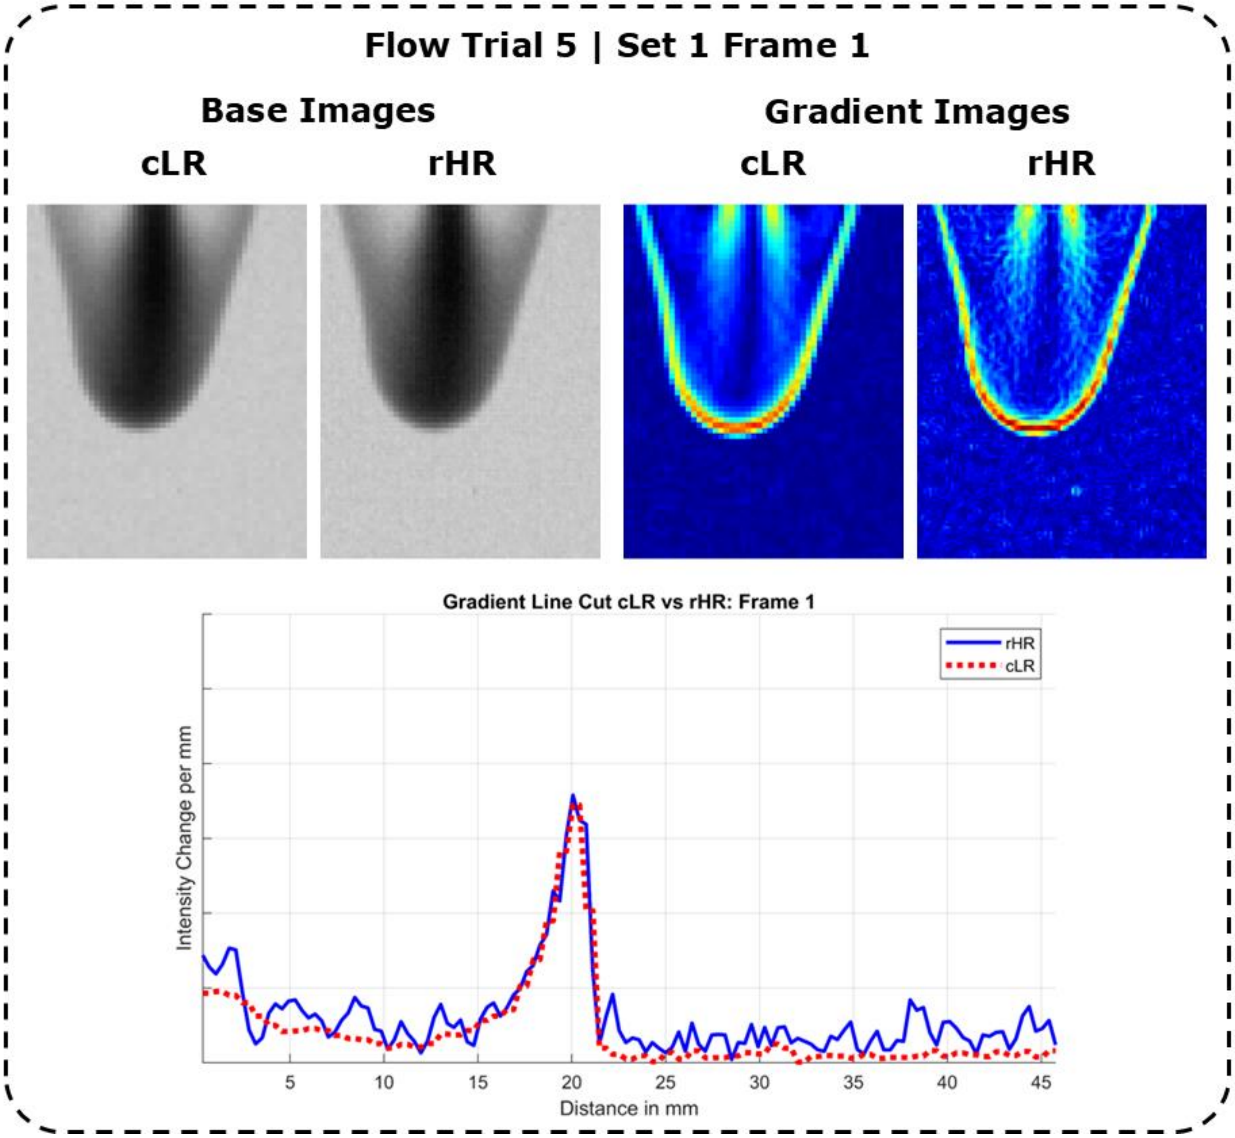


Supplemental Figure S17: Flow trial 5, set 1, frame 1 images, gradients, and gradient line cut.

Supplemental Figure S20 contains data from flow trial 5, set 1 frame 1 with an imaging frame rate of 40.05 FPS and a flow at 80 ml per hour. All images shown are cropped into the region of interest at the front of the flow. Captured low-resolution and reconstructed high-resolution images are shown along with their corresponding gradient. The gradient is normalized with respect to the pixel scale, 352 $\mu m$ for the cLR image and 176 $\mu m$ for the rHR image separately. We set the time for this initial frame to be 0 seconds. The gradient plot shows a vertical linecut of the center most column of pixels with the dashed red line denoting the cLR and the solid blue line denoting the rHR images. The x-axis shows the distance in mm from the exit of the nozzle. The y-axis is the intensity change normalized to the pixel scale with arbitrary units.

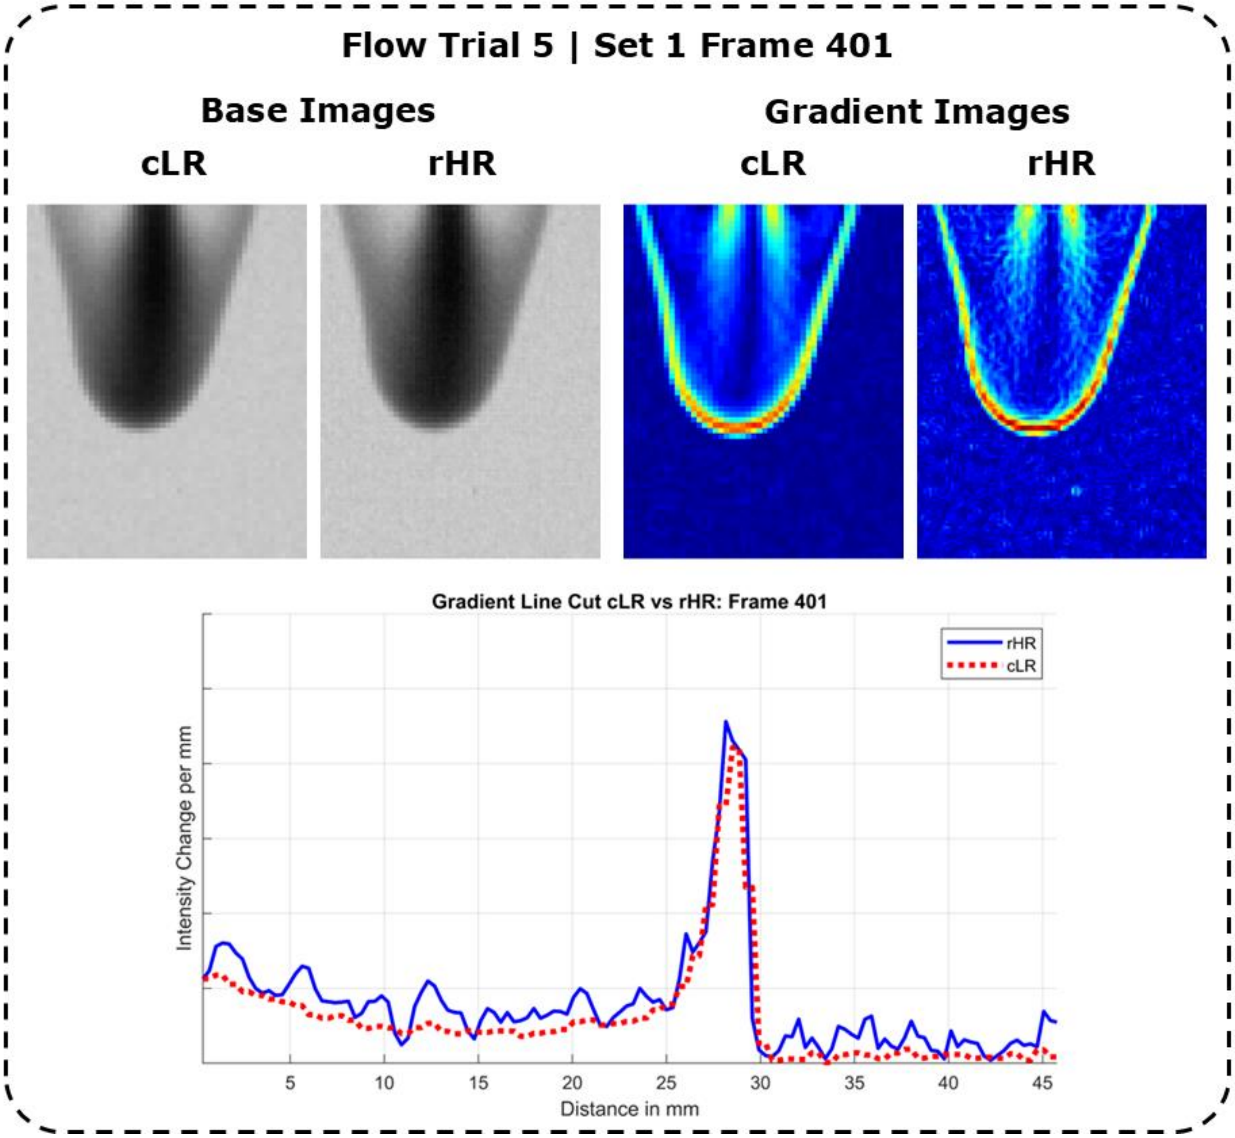


Supplemental Figure S18: Flow trial 5, set 1, frame 401 images, gradients, and gradient line cut.

Supplemental Figure S21 contains data from flow trial 5, set 1, frame 401 with an imaging frame rate of 40.05 FPS and a flow at 80 ml per hour. All images shown are cropped into the region of interest at the front of the flow. Captured low-resolution and reconstructed high-resolution images are shown along with their corresponding gradient. The gradient is normalized with respect to the pixel scale, 352 $\mu m$ for the cLR image and 176 $\mu m$ for the rHR image separately. This frame occurs 9.99 seconds after set 1, frame 1. The gradient plot shows a vertical linecut of the center most column of pixels with the dashed red line denoting the cLR and the solid blue line denoting the rHR images. The x-axis shows the distance in mm from the exit of the nozzle. The y-axis is the intensity change normalized to the pixel scale with arbitrary units.

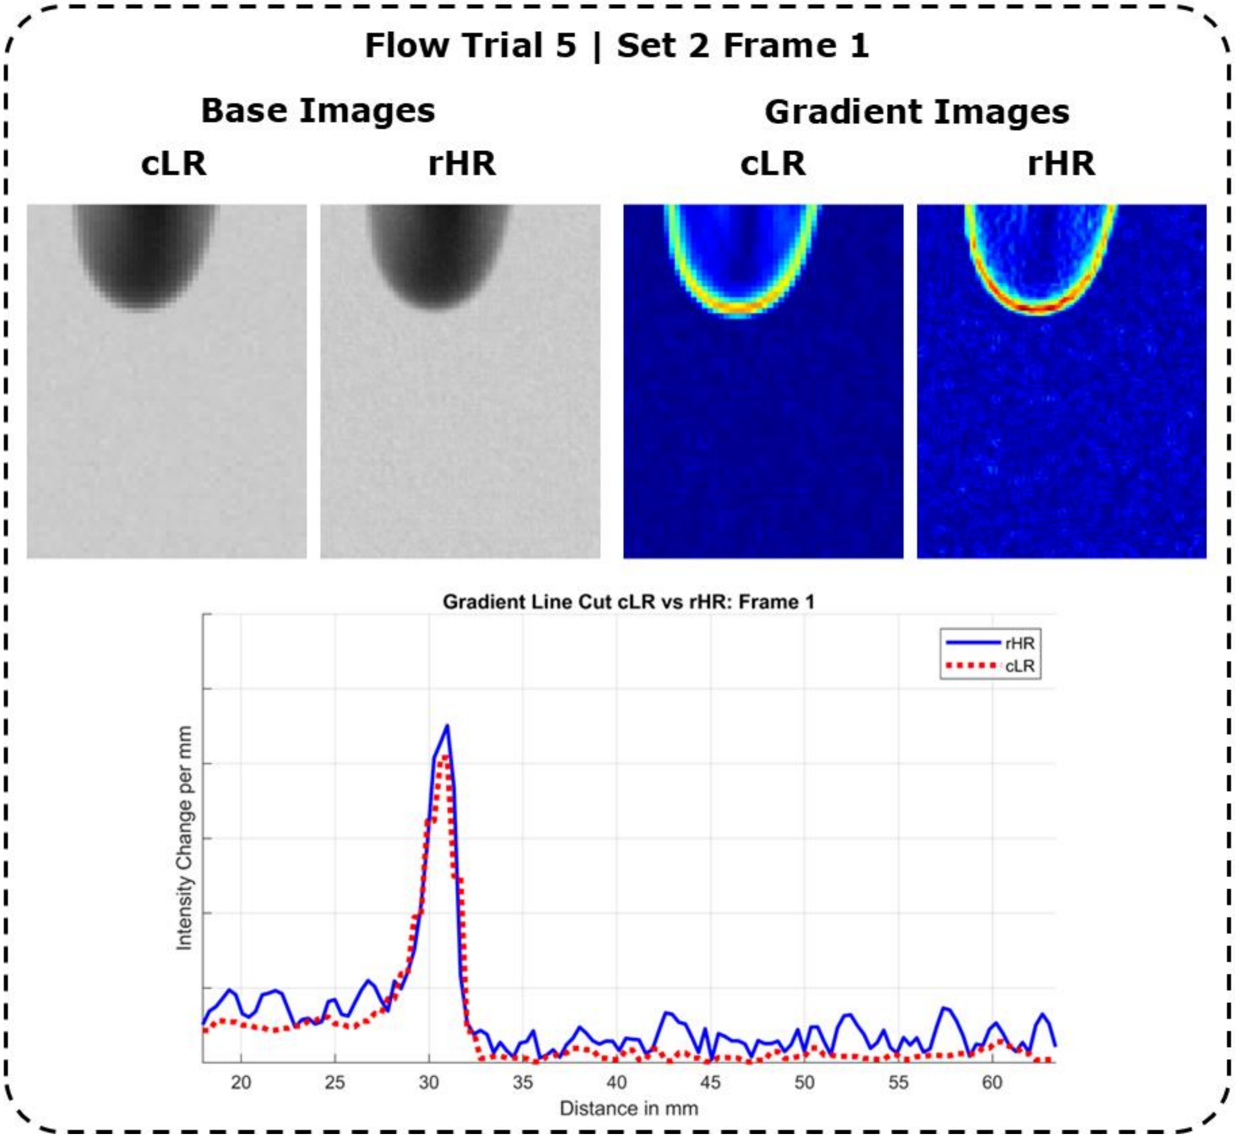


Supplemental Figure S19: Flow trial 5, set 2, frame 1 images, gradients, and gradient line cut.

Supplemental Figure S22 contains data from flow trial 5, set 2, frame 1 with an imaging frame rate of 40.05 FPS and a flow at 80 ml per hour. All images shown are cropped into the region of interest at the front of the flow. Captured low-resolution and reconstructed high-resolution images are shown along with their corresponding gradient. The gradient is normalized with respect to the pixel scale, 352 $\mu m$ for the cLR image and 176 $\mu m$ for the rHR image separately. This image occurs 12.06 seconds after set 1, frame 1. The gradient plot shows a vertical linecut of the center most column of pixels with the dashed red line denoting the cLR and the solid blue line denoting the rHR images. The x-axis shows the distance in mm from the exit of the nozzle. The y-axis is the intensity change normalized to the pixel scale with arbitrary units.

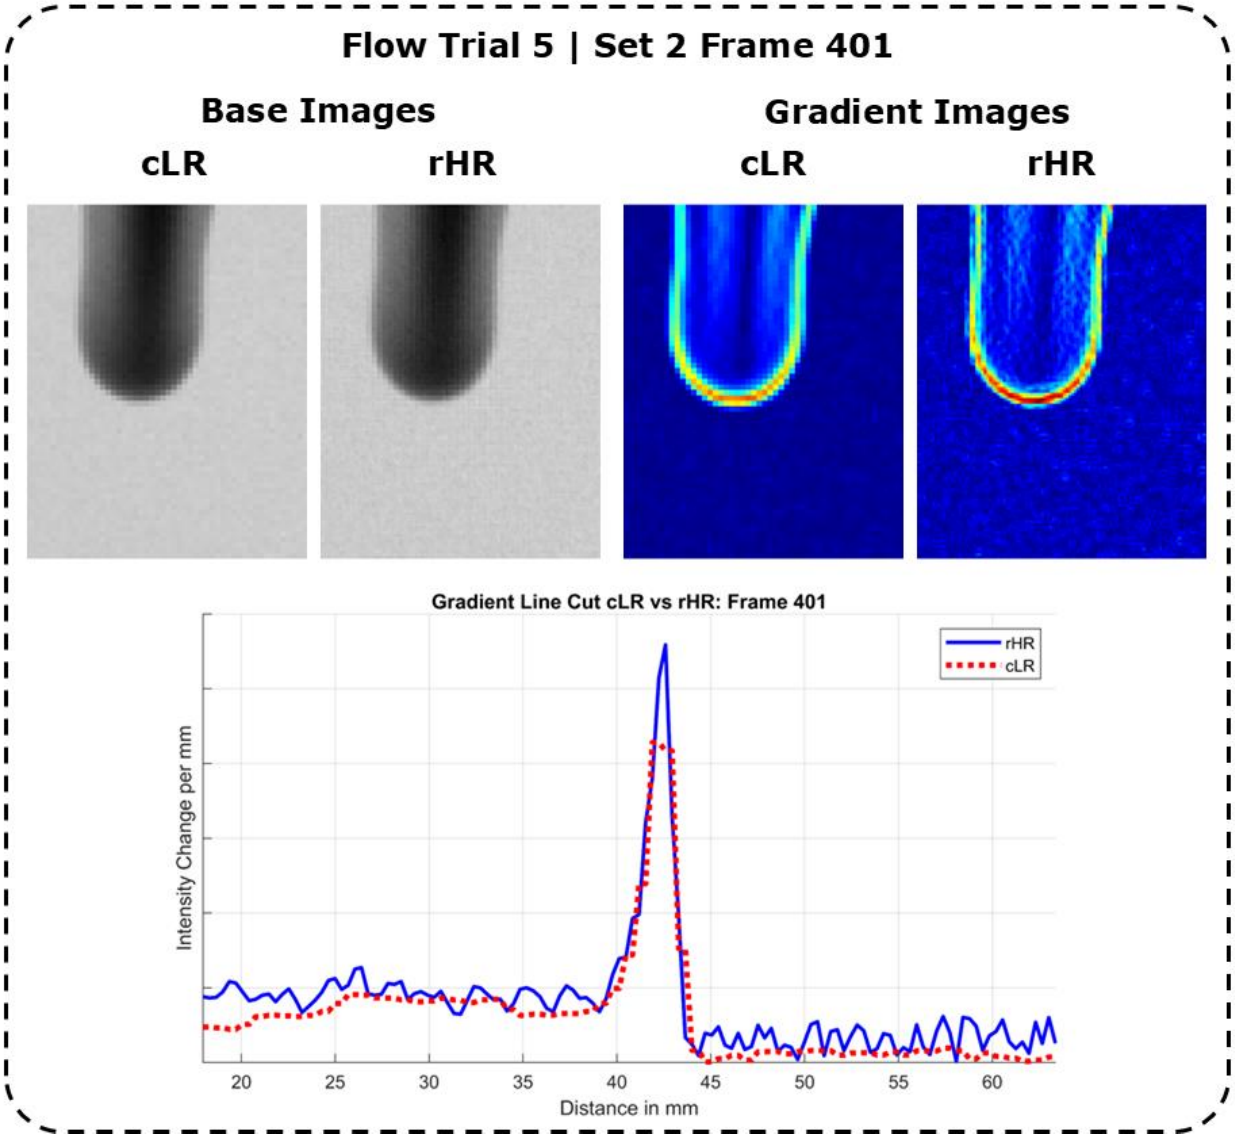


Supplemental Figure S20: Flow trial 5, set 2, frame 401 images, gradients, and gradient line cut.

Supplemental Figure S23 contains data from flow trial 5, set 2, frame 401 with an imaging frame rate of 40.05 FPS and a flow at 80 ml per hour. All images shown are cropped into the region of interest at the front of the flow. Captured low-resolution and reconstructed high-resolution images are shown along with their corresponding gradient. The gradient is normalized with respect to the pixel scale, 352 $\mu m$ for the cLR image and 176 $\mu m$ for the rHR image separately. This image occurs 22.05 seconds after set 1, frame 1. The gradient plot shows a vertical linecut of the center most column of pixels with the dashed red line denoting the cLR and the solid blue line denoting the rHR images. The x-axis shows the distance in mm from the exit of the nozzle. The y-axis is the intensity change normalized to the pixel scale with arbitrary units.

**Flow Trial 6**

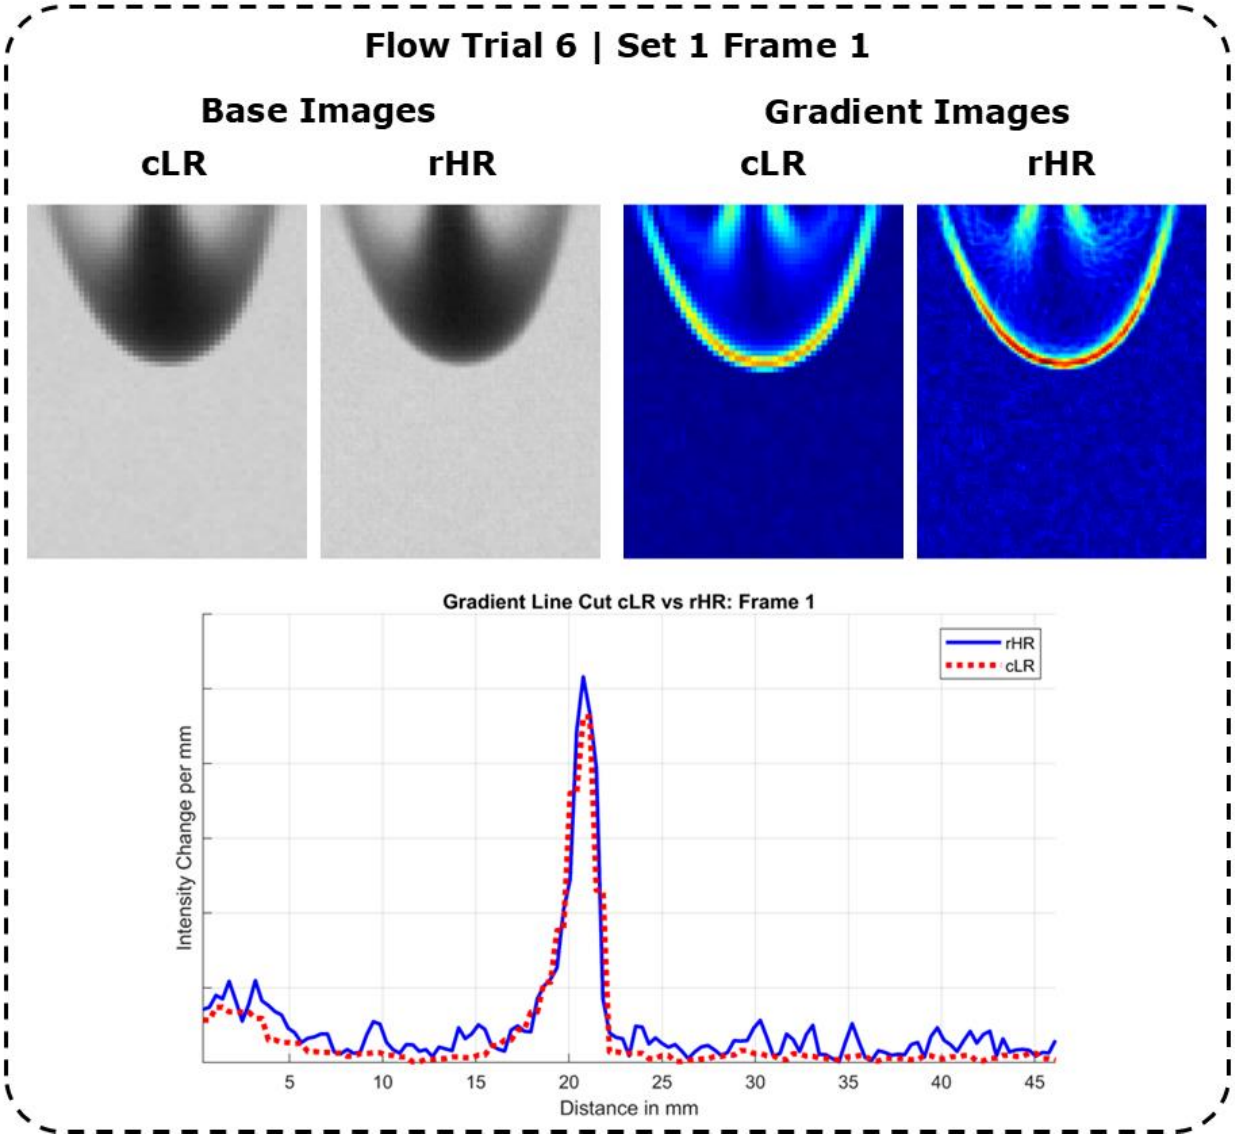


Supplemental Figure S21: Flow trial 6, set 1, frame 1 images, gradients, and gradient line cut.

Supplemental Figure S24 contains data from flow trial 6, set 1 frame 1 with an imaging frame rate of 40.05 FPS and a flow at 100 ml per hour. All images shown are cropped into the region of interest at the front of the flow. Captured low-resolution and reconstructed high-resolution images are shown along with their corresponding gradient. The gradient is normalized with respect to the pixel scale, 352 $\mu m$ for the cLR image and 176 $\mu m$ for the rHR image separately. We set the time for this initial frame to be 0 seconds. The gradient plot shows a vertical linecut of the center most column of pixels with the dashed red line denoting the cLR and the solid blue line denoting the rHR images. The x-axis shows the distance in mm from the exit of the nozzle. The y-axis is the intensity change normalized to the pixel scale with arbitrary units.

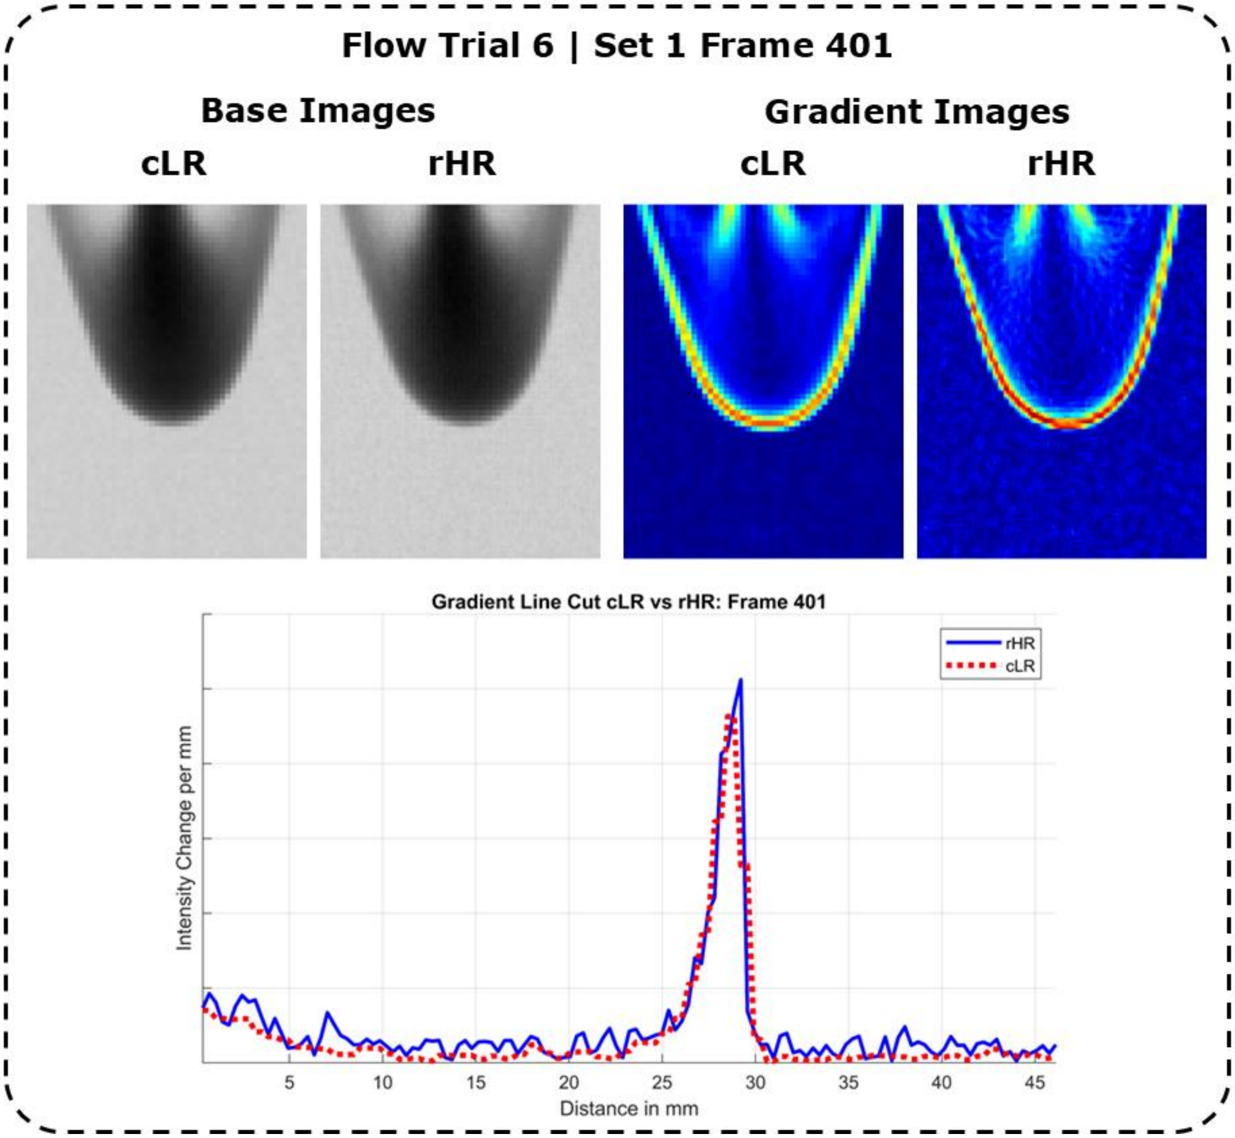


Supplemental Figure S22: Flow trial 6, set 1, frame 401 images, gradients, and gradient line cut.

Supplemental Figure S25 contains data from flow trial 6, set 1, frame 401 with an imaging frame rate of 40.05 FPS and a flow at 100 ml per hour. All images shown are cropped into the region of interest at the front of the flow. Captured low-resolution and reconstructed high-resolution images are shown along with their corresponding gradient. The gradient is normalized with respect to the pixel scale, 352 $\mu m$ for the cLR image and 176 $\mu m$ for the rHR image separately. This frame occurs 9.99 seconds after set 1, frame 1. The gradient plot shows a vertical linecut of the center most column of pixels with the dashed red line denoting the cLR and the solid blue line denoting the rHR images. The x-axis shows the distance in mm from the exit of the nozzle. The y-axis is the intensity change normalized to the pixel scale with arbitrary units.

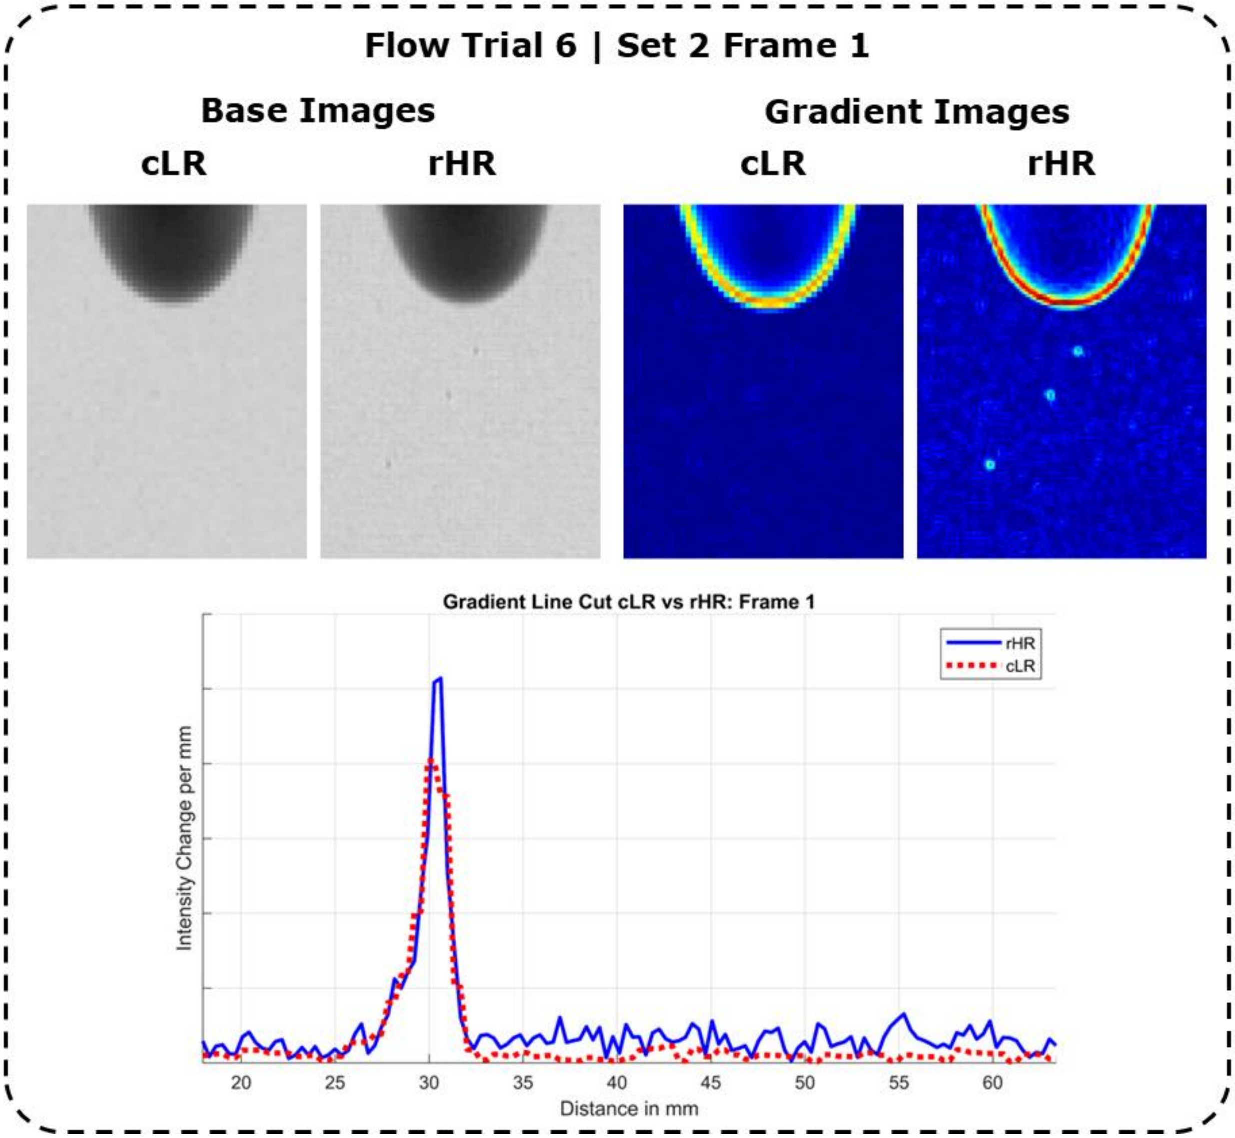


Supplemental Figure S23: Flow trial 6, set 2, frame 1 images, gradients, and gradient line cut.

Supplemental Figure S26 contains data from flow trial 6, set 2, frame 1 with an imaging frame rate of 40.05 FPS and a flow at 100 ml per hour. All images shown are cropped into the region of interest at the front of the flow. Captured low-resolution and reconstructed high-resolution images are shown along with their corresponding gradient. The gradient is normalized with respect to the pixel scale, 352 $\mu m$ for the cLR image and 176 $\mu m$ for the rHR image separately. This image occurs 11.74 seconds after set 1, frame 1. The gradient plot shows a vertical linecut of the center most column of pixels with the dashed red line denoting the cLR and the solid blue line denoting the rHR images. The x-axis shows the distance in mm from the exit of the nozzle. The y-axis is the intensity change normalized to the pixel scale with arbitrary units.

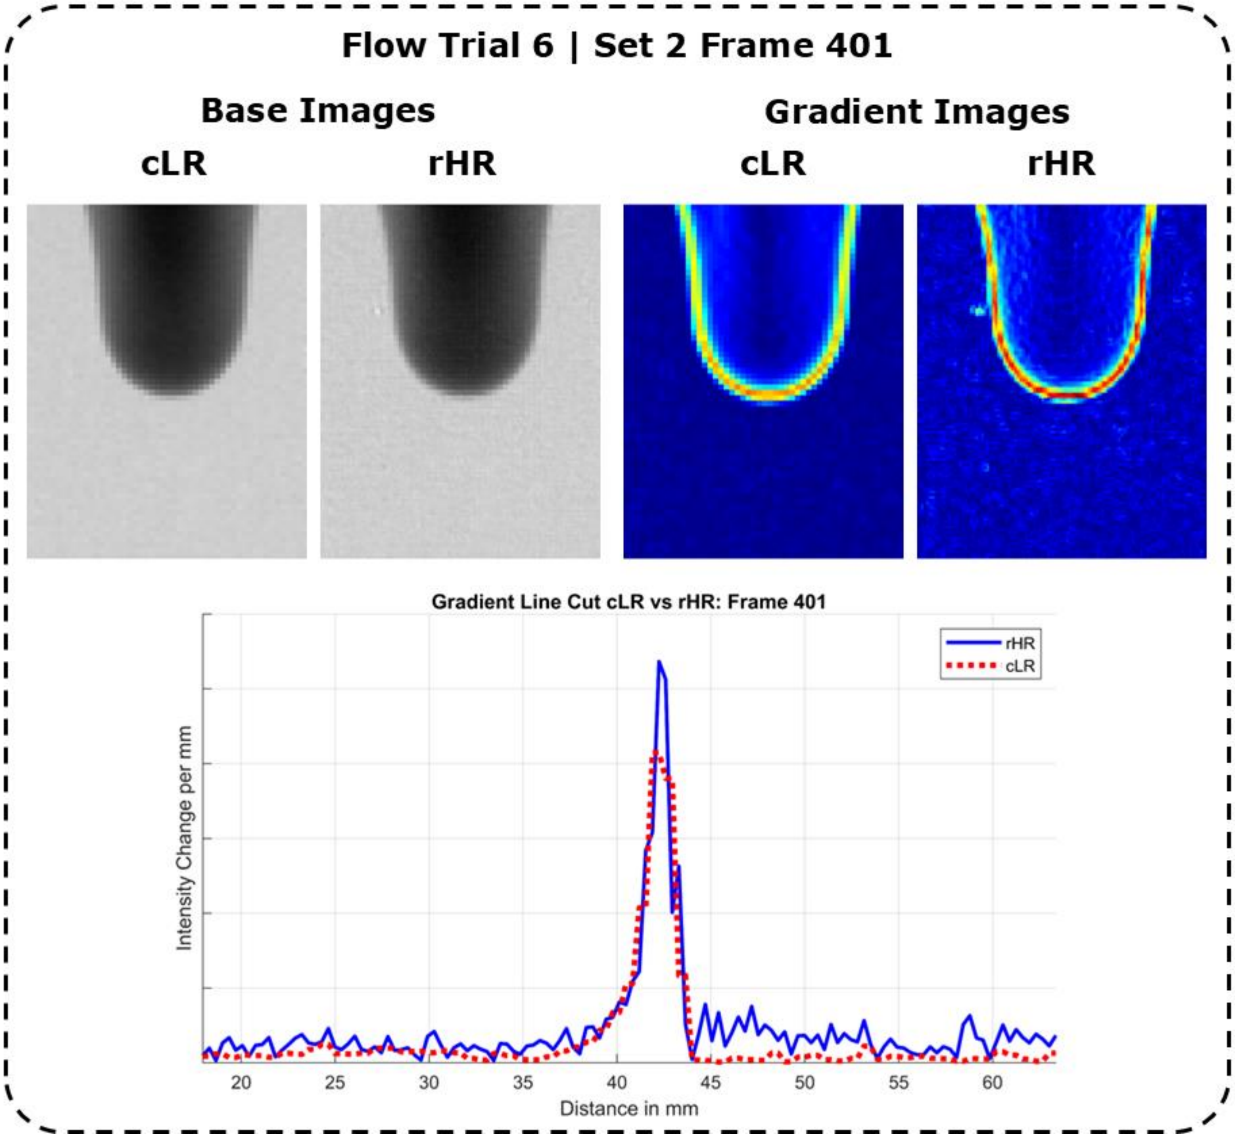


Supplemental Figure S24: Flow trial 6, set 2, frame 401 images, gradients, and gradient line cut.

Supplemental Figure S27 contains data from flow trial 6, set 2, frame 401 with an imaging frame rate of 40.05 FPS and a flow at 100 ml per hour. All images shown are cropped into the region of interest at the front of the flow. Captured low-resolution and reconstructed high-resolution images are shown along with their corresponding gradient. The gradient is normalized with respect to the pixel scale, 352 $\mu m$ for the cLR image and 176 $\mu m$ for the rHR image separately. This image occurs 21.72 seconds after set 1, frame 1. The gradient plot shows a vertical linecut of the center most column of pixels with the dashed red line denoting the cLR and the solid blue line denoting the rHR images. The x-axis shows the distance in mm from the exit of the nozzle. The y-axis is the intensity change normalized to the pixel scale with arbitrary units.

**Flow Trial 7**

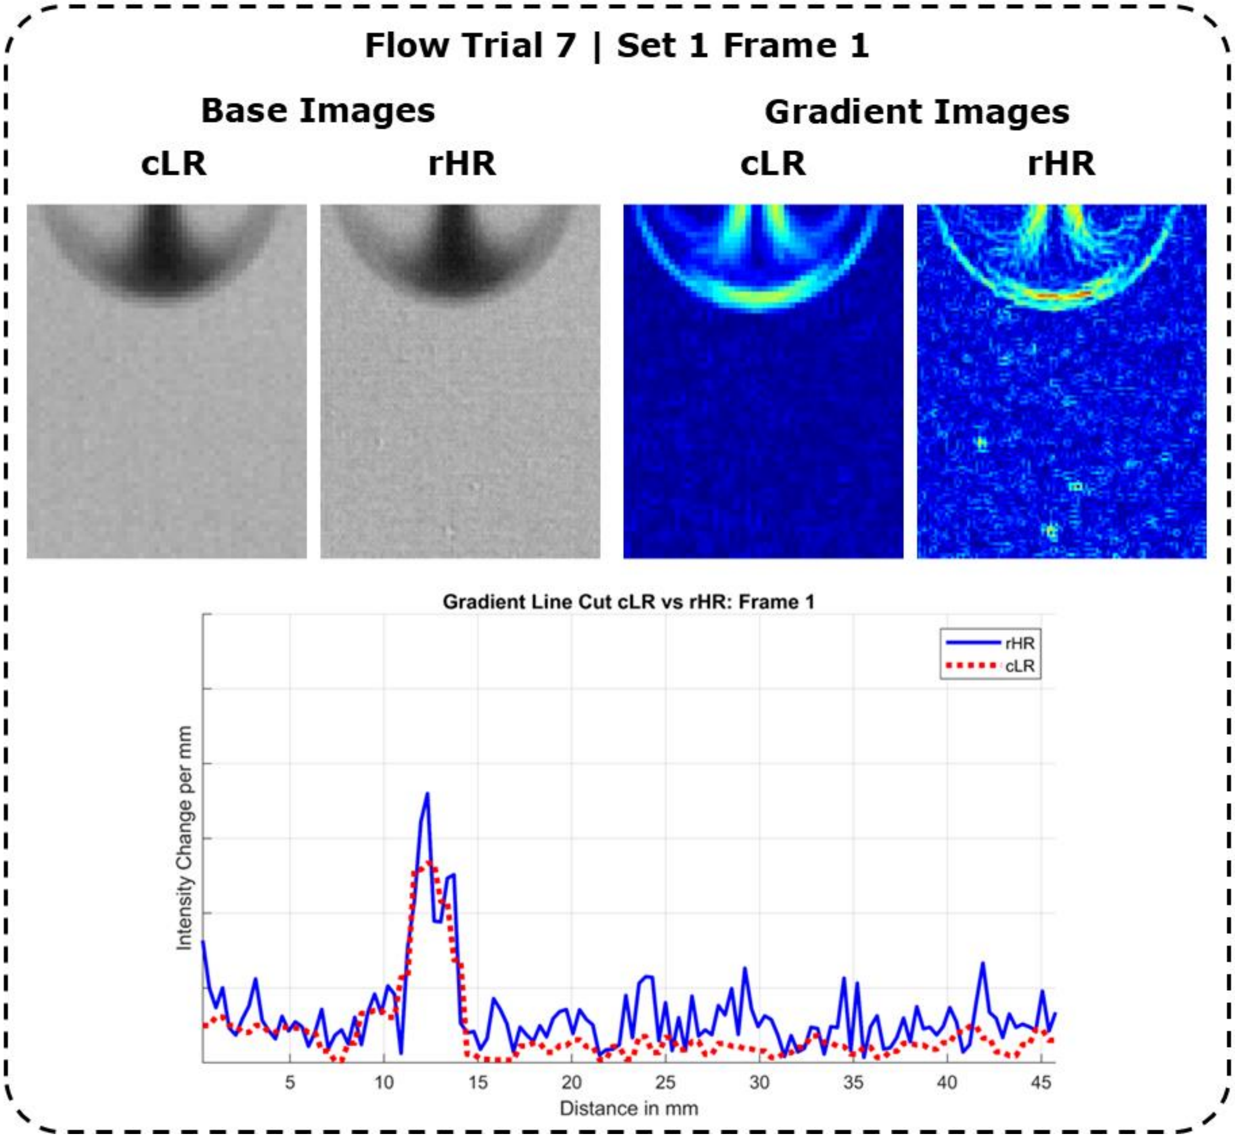


Supplemental Figure S25: Flow trial 7, set 1, frame 1 images, gradients, and gradient line cut.

Supplemental Figure S28 contains data from flow trial 7, set 1 frame 1 with an imaging frame rate of 40.05 FPS and a flow at 120 ml per hour. All images shown are cropped into the region of interest at the front of the flow. Captured low-resolution and reconstructed high-resolution images are shown along with their corresponding gradient. The gradient is normalized with respect to the pixel scale, 352 $\mu m$ for the cLR image and 176 $\mu m$ for the rHR image separately. We set the time for this initial frame to be 0 seconds. The gradient plot shows a vertical linecut of the center most column of pixels with the dashed red line denoting the cLR and the solid blue line denoting the rHR images. The x-axis shows the distance in mm from the exit of the nozzle. The y-axis is the intensity change normalized to the pixel scale with arbitrary units.

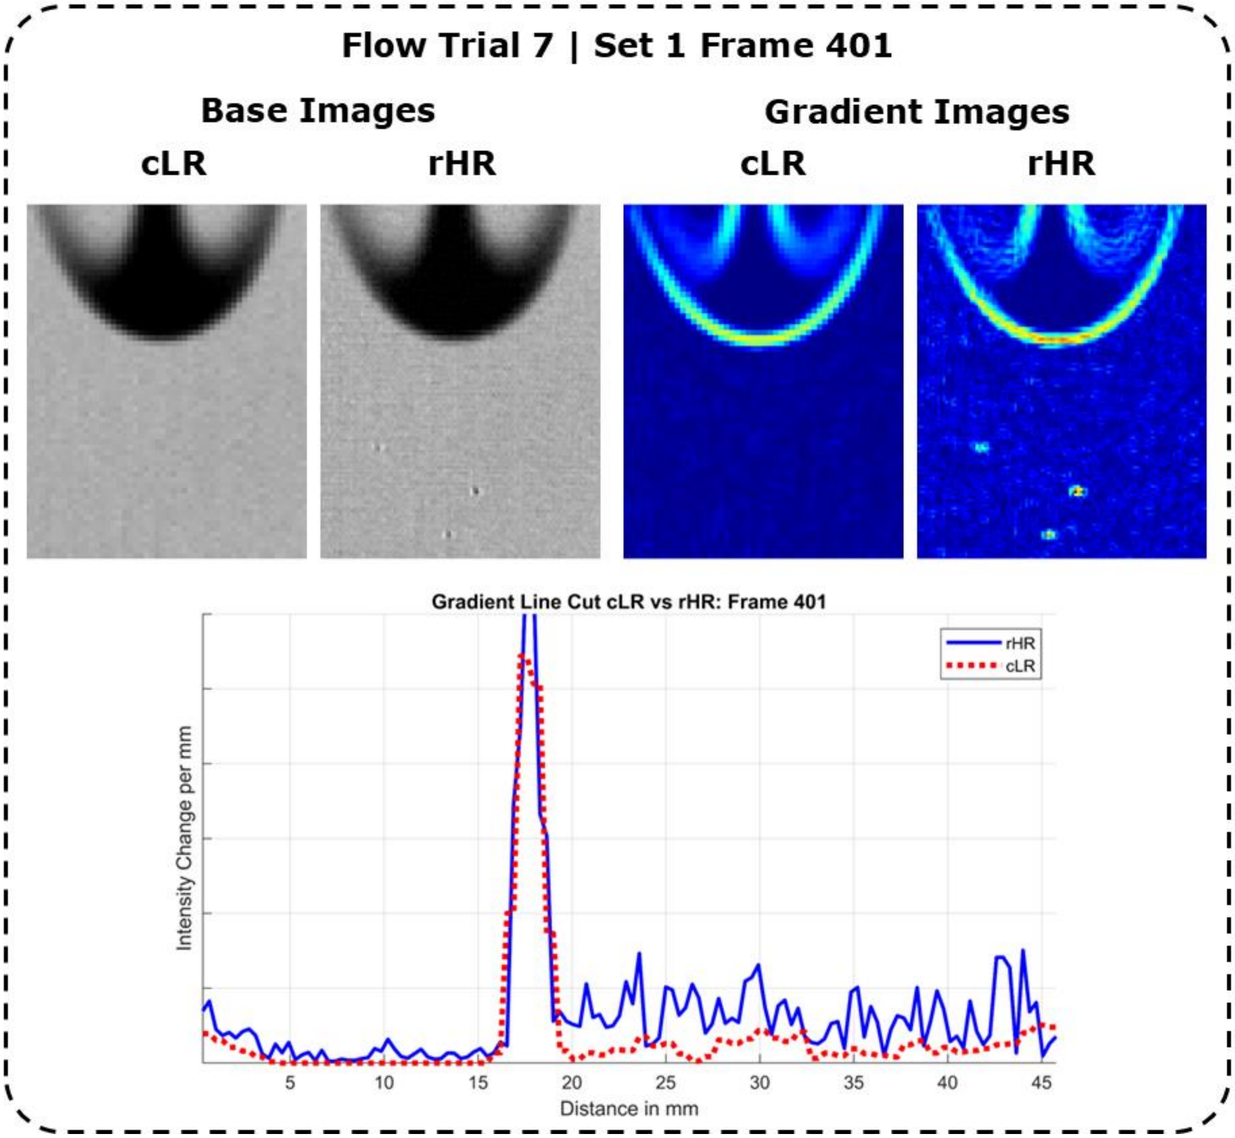


Supplemental Figure S26: Flow trial 7, set 1, frame 401 images, gradients, and gradient line cut.

Supplemental Figure S29 contains data from flow trial 7, set 1, frame 401 with an imaging frame rate of 40.05 FPS and a flow at 120 ml per hour. All images shown are cropped into the region of interest at the front of the flow. Captured low-resolution and reconstructed high-resolution images are shown along with their corresponding gradient. The gradient is normalized with respect to the pixel scale, 352 $\mu m$ for the cLR image and 176 $\mu m$ for the rHR image separately. This frame occurs 9.99 seconds after set 1, frame 1. The gradient plot shows a vertical linecut of the center most column of pixels with the dashed red line denoting the cLR and the solid blue line denoting the rHR images. The x-axis shows the distance in mm from the exit of the nozzle. The y-axis is the intensity change normalized to the pixel scale with arbitrary units.

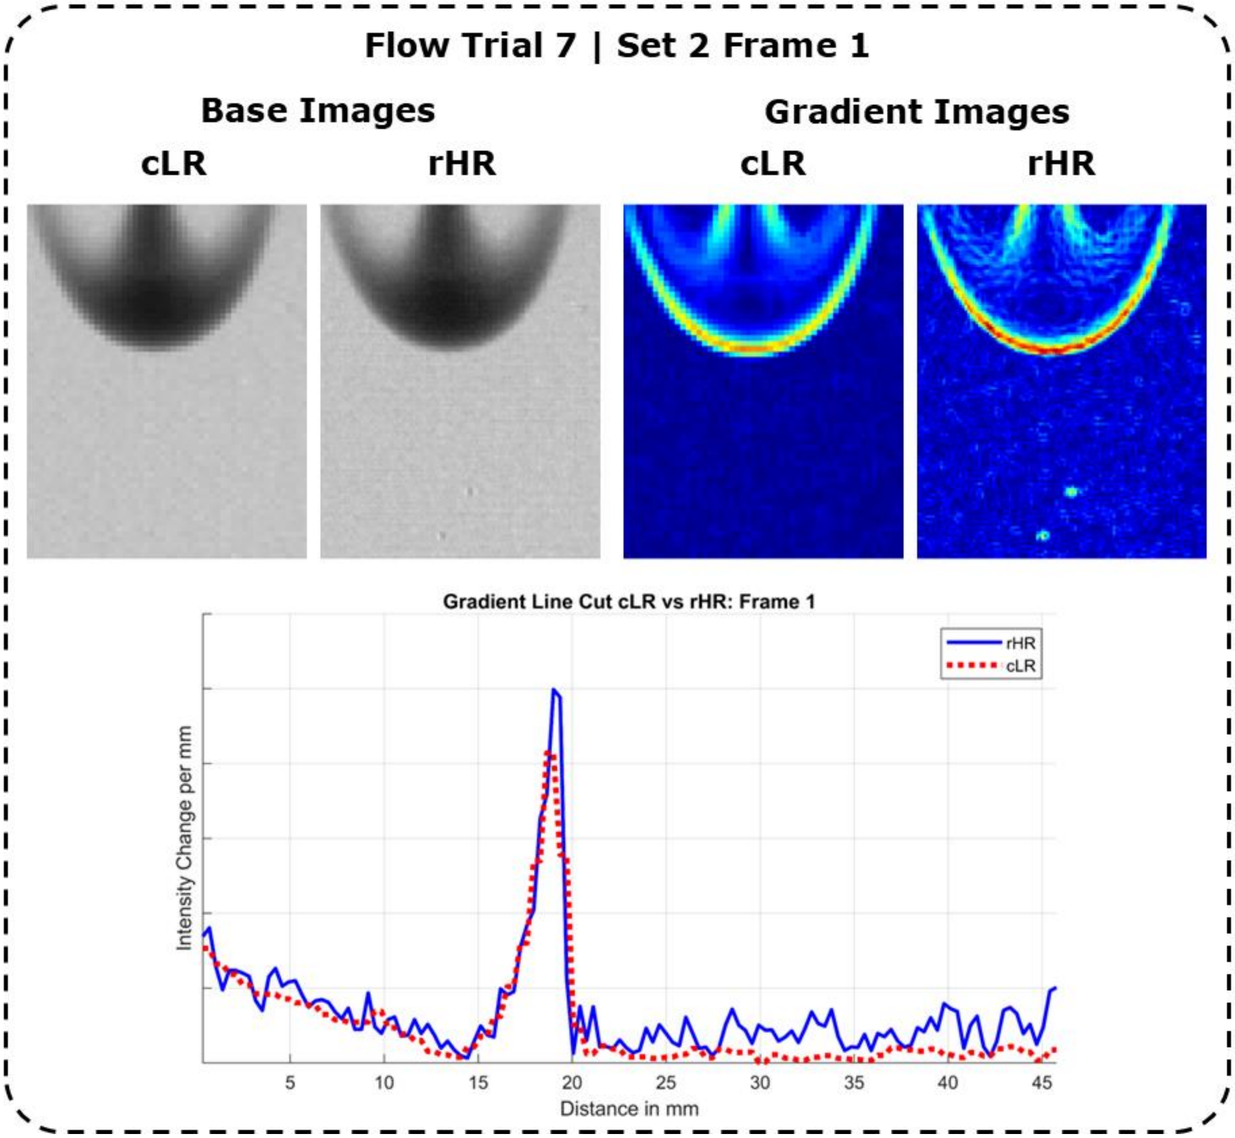


Supplemental Figure S27: Flow trial 7, set 2, frame 1 images, gradients, and gradient line cut.

Supplemental Figure S30 contains data from flow trial 7, set 2, frame 1 with an imaging frame rate of 40.05 FPS and a flow at 120 ml per hour. All images shown are cropped into the region of interest at the front of the flow. Captured low-resolution and reconstructed high-resolution images are shown along with their corresponding gradient. The gradient is normalized with respect to the pixel scale, 352 $\mu m$ for the cLR image and 176 $\mu m$ for the rHR image separately. This image occurs 11.84 seconds after set 1, frame 1. The gradient plot shows a vertical linecut of the center most column of pixels with the dashed red line denoting the cLR and the solid blue line denoting the rHR images. The x-axis shows the distance in mm from the exit of the nozzle. The y-axis is the intensity change normalized to the pixel scale with arbitrary units.

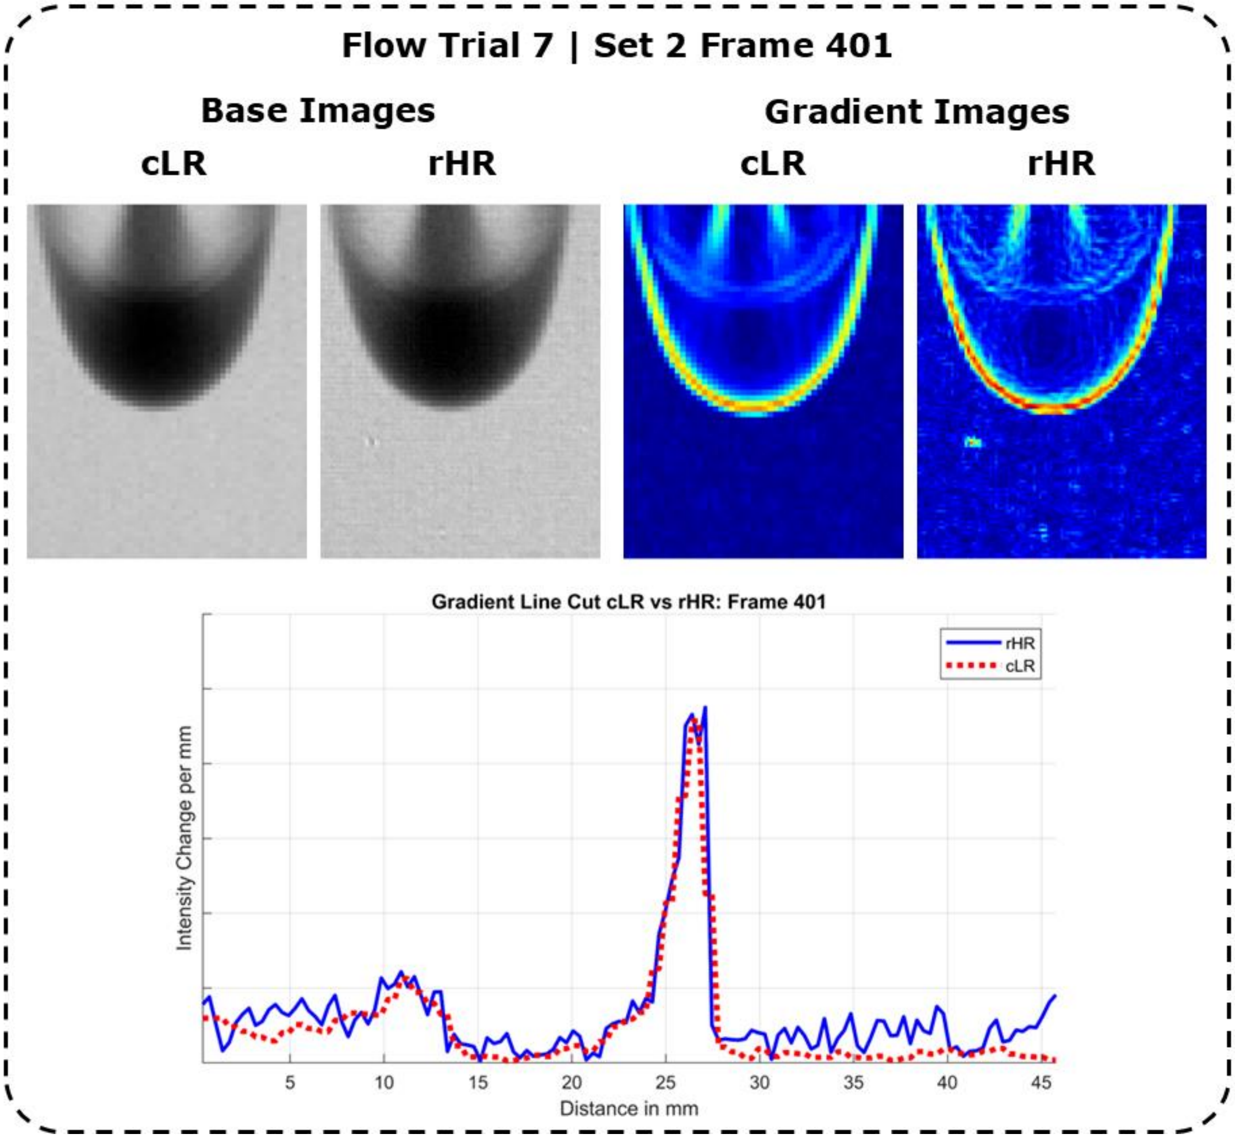


Supplemental Figure S28: Flow trial 7, set 2, frame 401 images, gradients, and gradient line cut.

Supplemental Figure S31 contains data from flow trial 7, set 2, frame 401 with an imaging frame rate of 40.05 FPS and a flow at 120 ml per hour. All images shown are cropped into the region of interest at the front of the flow. Captured low-resolution and reconstructed high-resolution images are shown along with their corresponding gradient. The gradient is normalized with respect to the pixel scale, 352 $\mu m$ for the cLR image and 176 $\mu m$ for the rHR image separately. This image occurs 21.82 seconds after set 1, frame 1. The gradient plot shows a vertical linecut of the center most column of pixels with the dashed red line denoting the cLR and the solid blue line denoting the rHR images. The x-axis shows the distance in mm from the exit of the nozzle. The y-axis is the intensity change normalized to the pixel scale with arbitrary units.
